# Supplementary material for: Chemically Homogeneous Evolution: A rapid population synthesis approach
Source: arXiv:2010.00002 source file (2021-05-02)
Supplement: Supplementary file 1 [file appendix-CDFgaps.tex]

\onecolumn
\begin{multicols}{2}
\section{CDF coverage}\label{sec:CDFGaps}

\ilya{[So it is sampling uncertainty alone that is responsible?  And the error bars in earlier figures are just under-estimated?  This seems to call for drawing more samples -- can we use AIS?  And not binning in such narrow bins, but smoothing the distributions for more accurate visuals (wider bins, KDEs, plotting CDFs)...  Good to have this investigation, probably should not be included in the paper.]} 

Figure~\ref{fig:cumulativeMchirpLigo} shows evidence of gaps in the constructed \ac{CHE} \acp{CDF}. These gaps coincide with low points in the corresponding \ac{PDF}(Figure~\ref{fig:chirp_mass_O1_fWR1_0}, dashed line). Figure~\ref{fig:Mchirp_O1_fWR1_0_all} shows the contribution to Figure~\ref{fig:chirp_mass_O1_fWR1_0} of the grid of metallicities used in our simulations, and it is apparent that the low points, or gaps, in both distributions (full population and \ac{CHE} only) are not due to coarseness of the metallicity grid - that is, the gaps in the \acp{PDF} are not caused by gaps in the metallicity grid.

\end{multicols}

\begin{multicols}{2}
\end{multicols}
\begin{multicols}{2}
\includegraphics[viewport = 5 5 555 507, width=7.84cm, clip]
{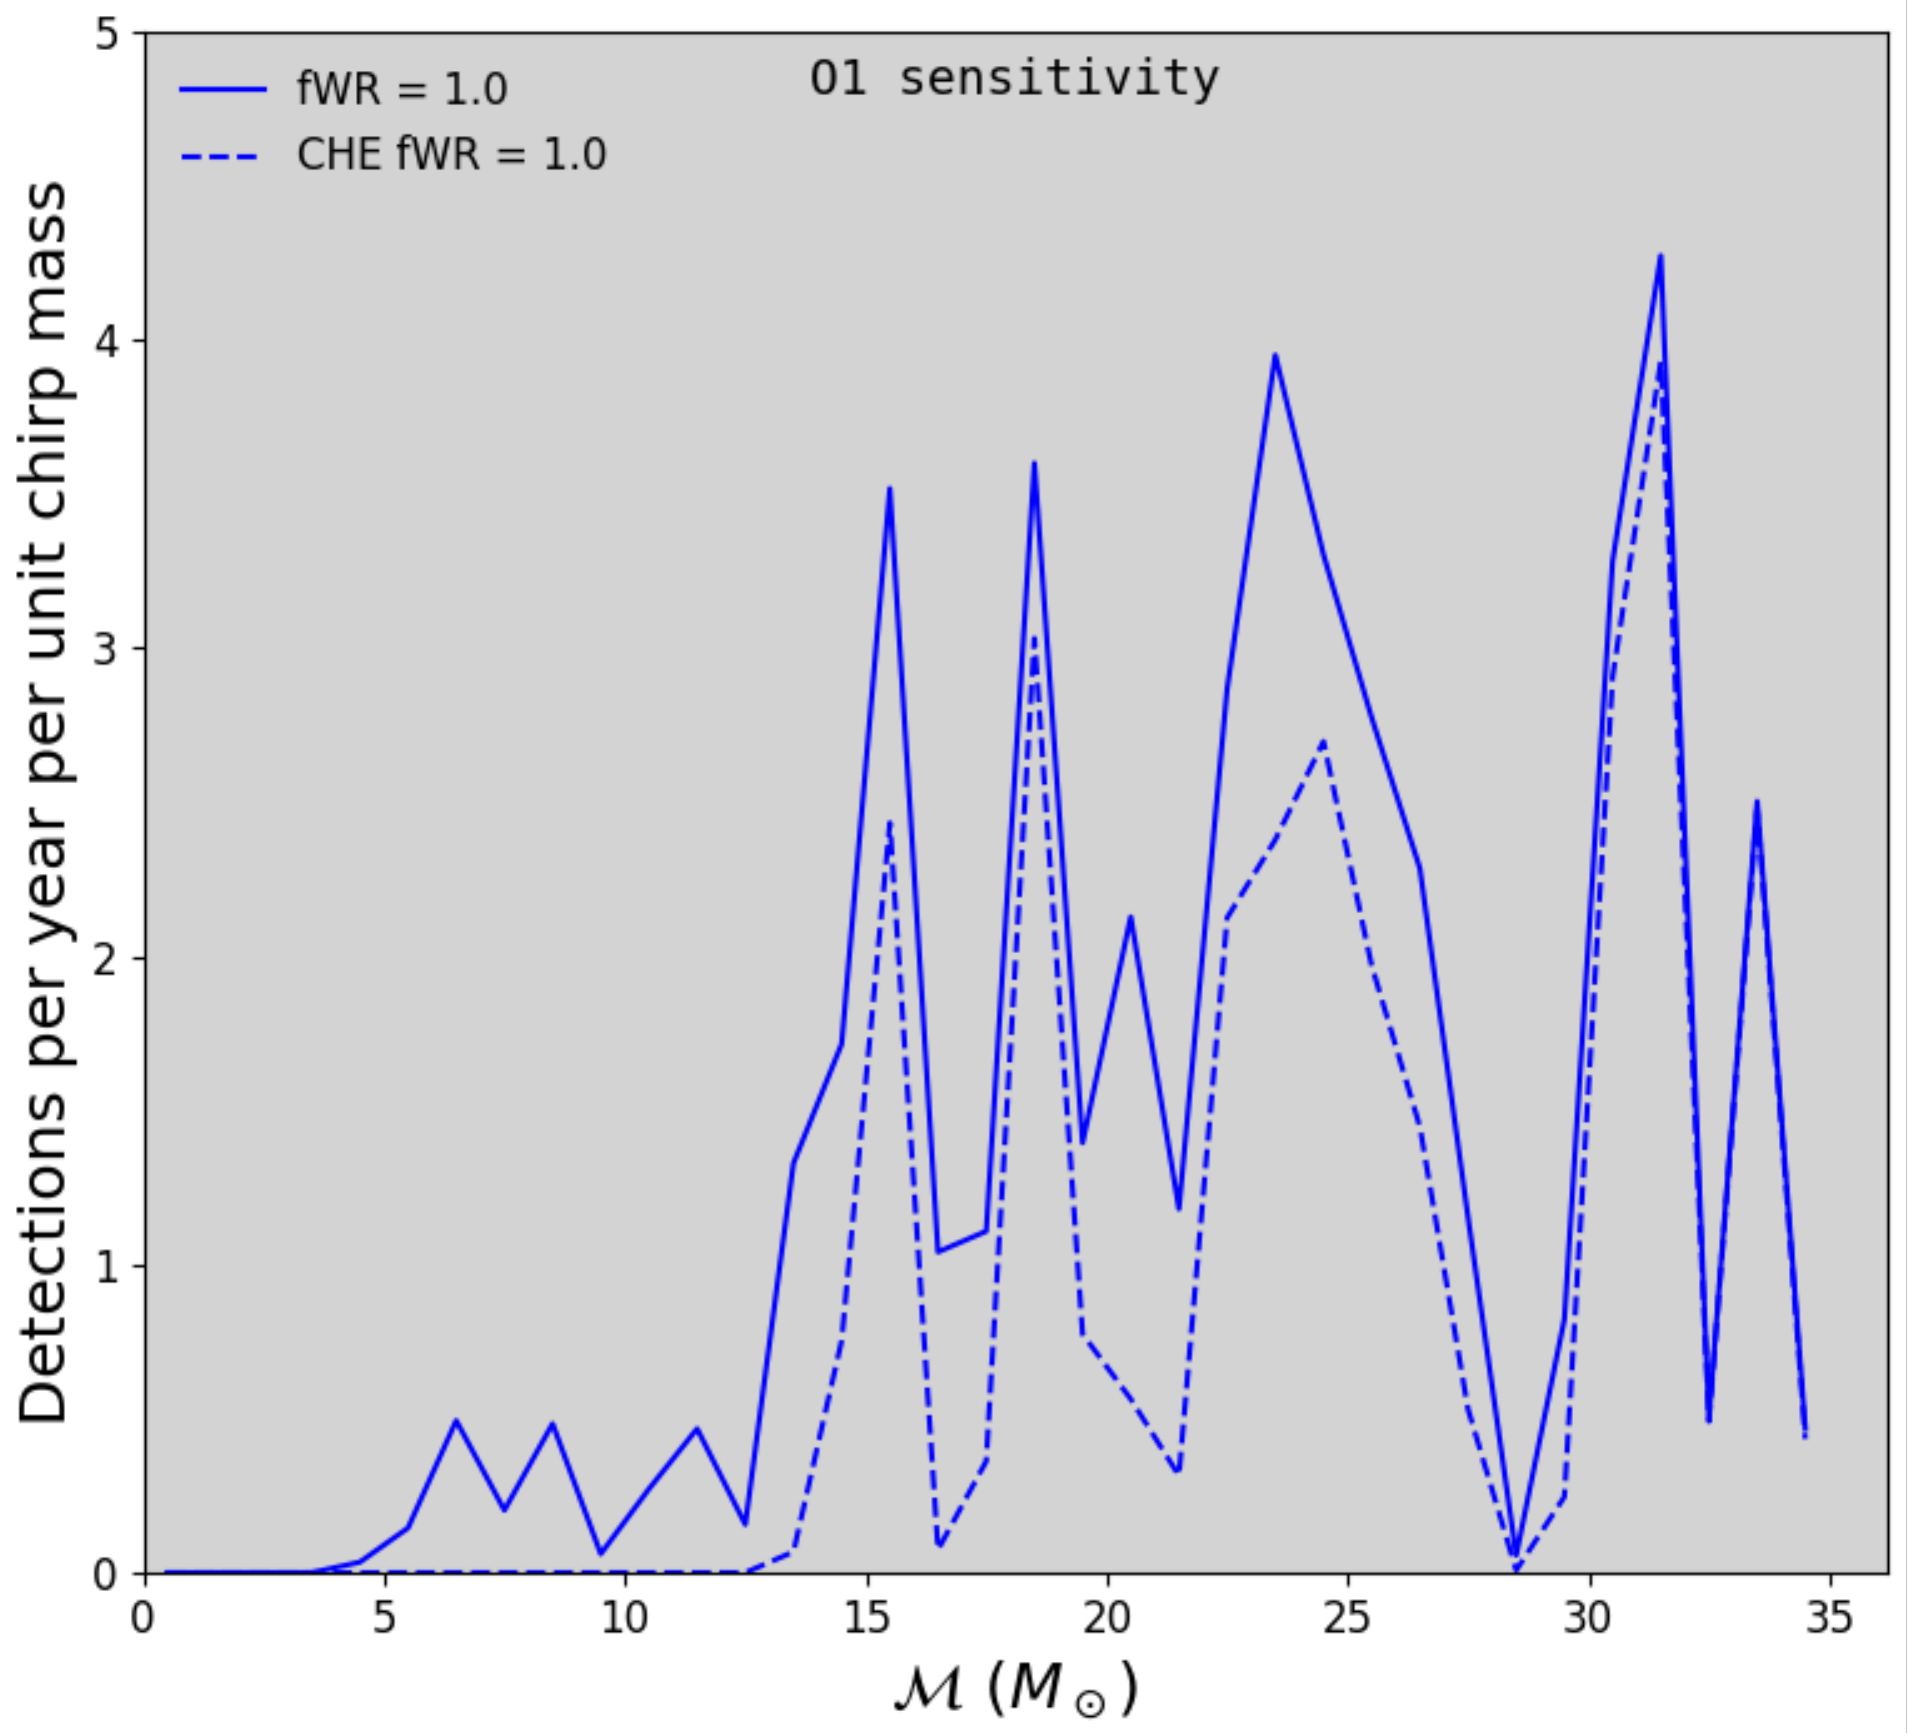}
\captionof{figure}{Predicted chirp mass distributions of \ac{BBH} mergers detectable at aLIGO observing runs 1 and 2 sensitivity, for $f_{wr}=1.0$.  Masses are in the source reference frame.  The solid line shows the full population distribution; the dashed line the distribution for \ac{CHE} systems only.}
\label{fig:chirp_mass_O1_fWR1_0}

\includegraphics[viewport = 5 5 600 510, width=8.45cm, clip]
{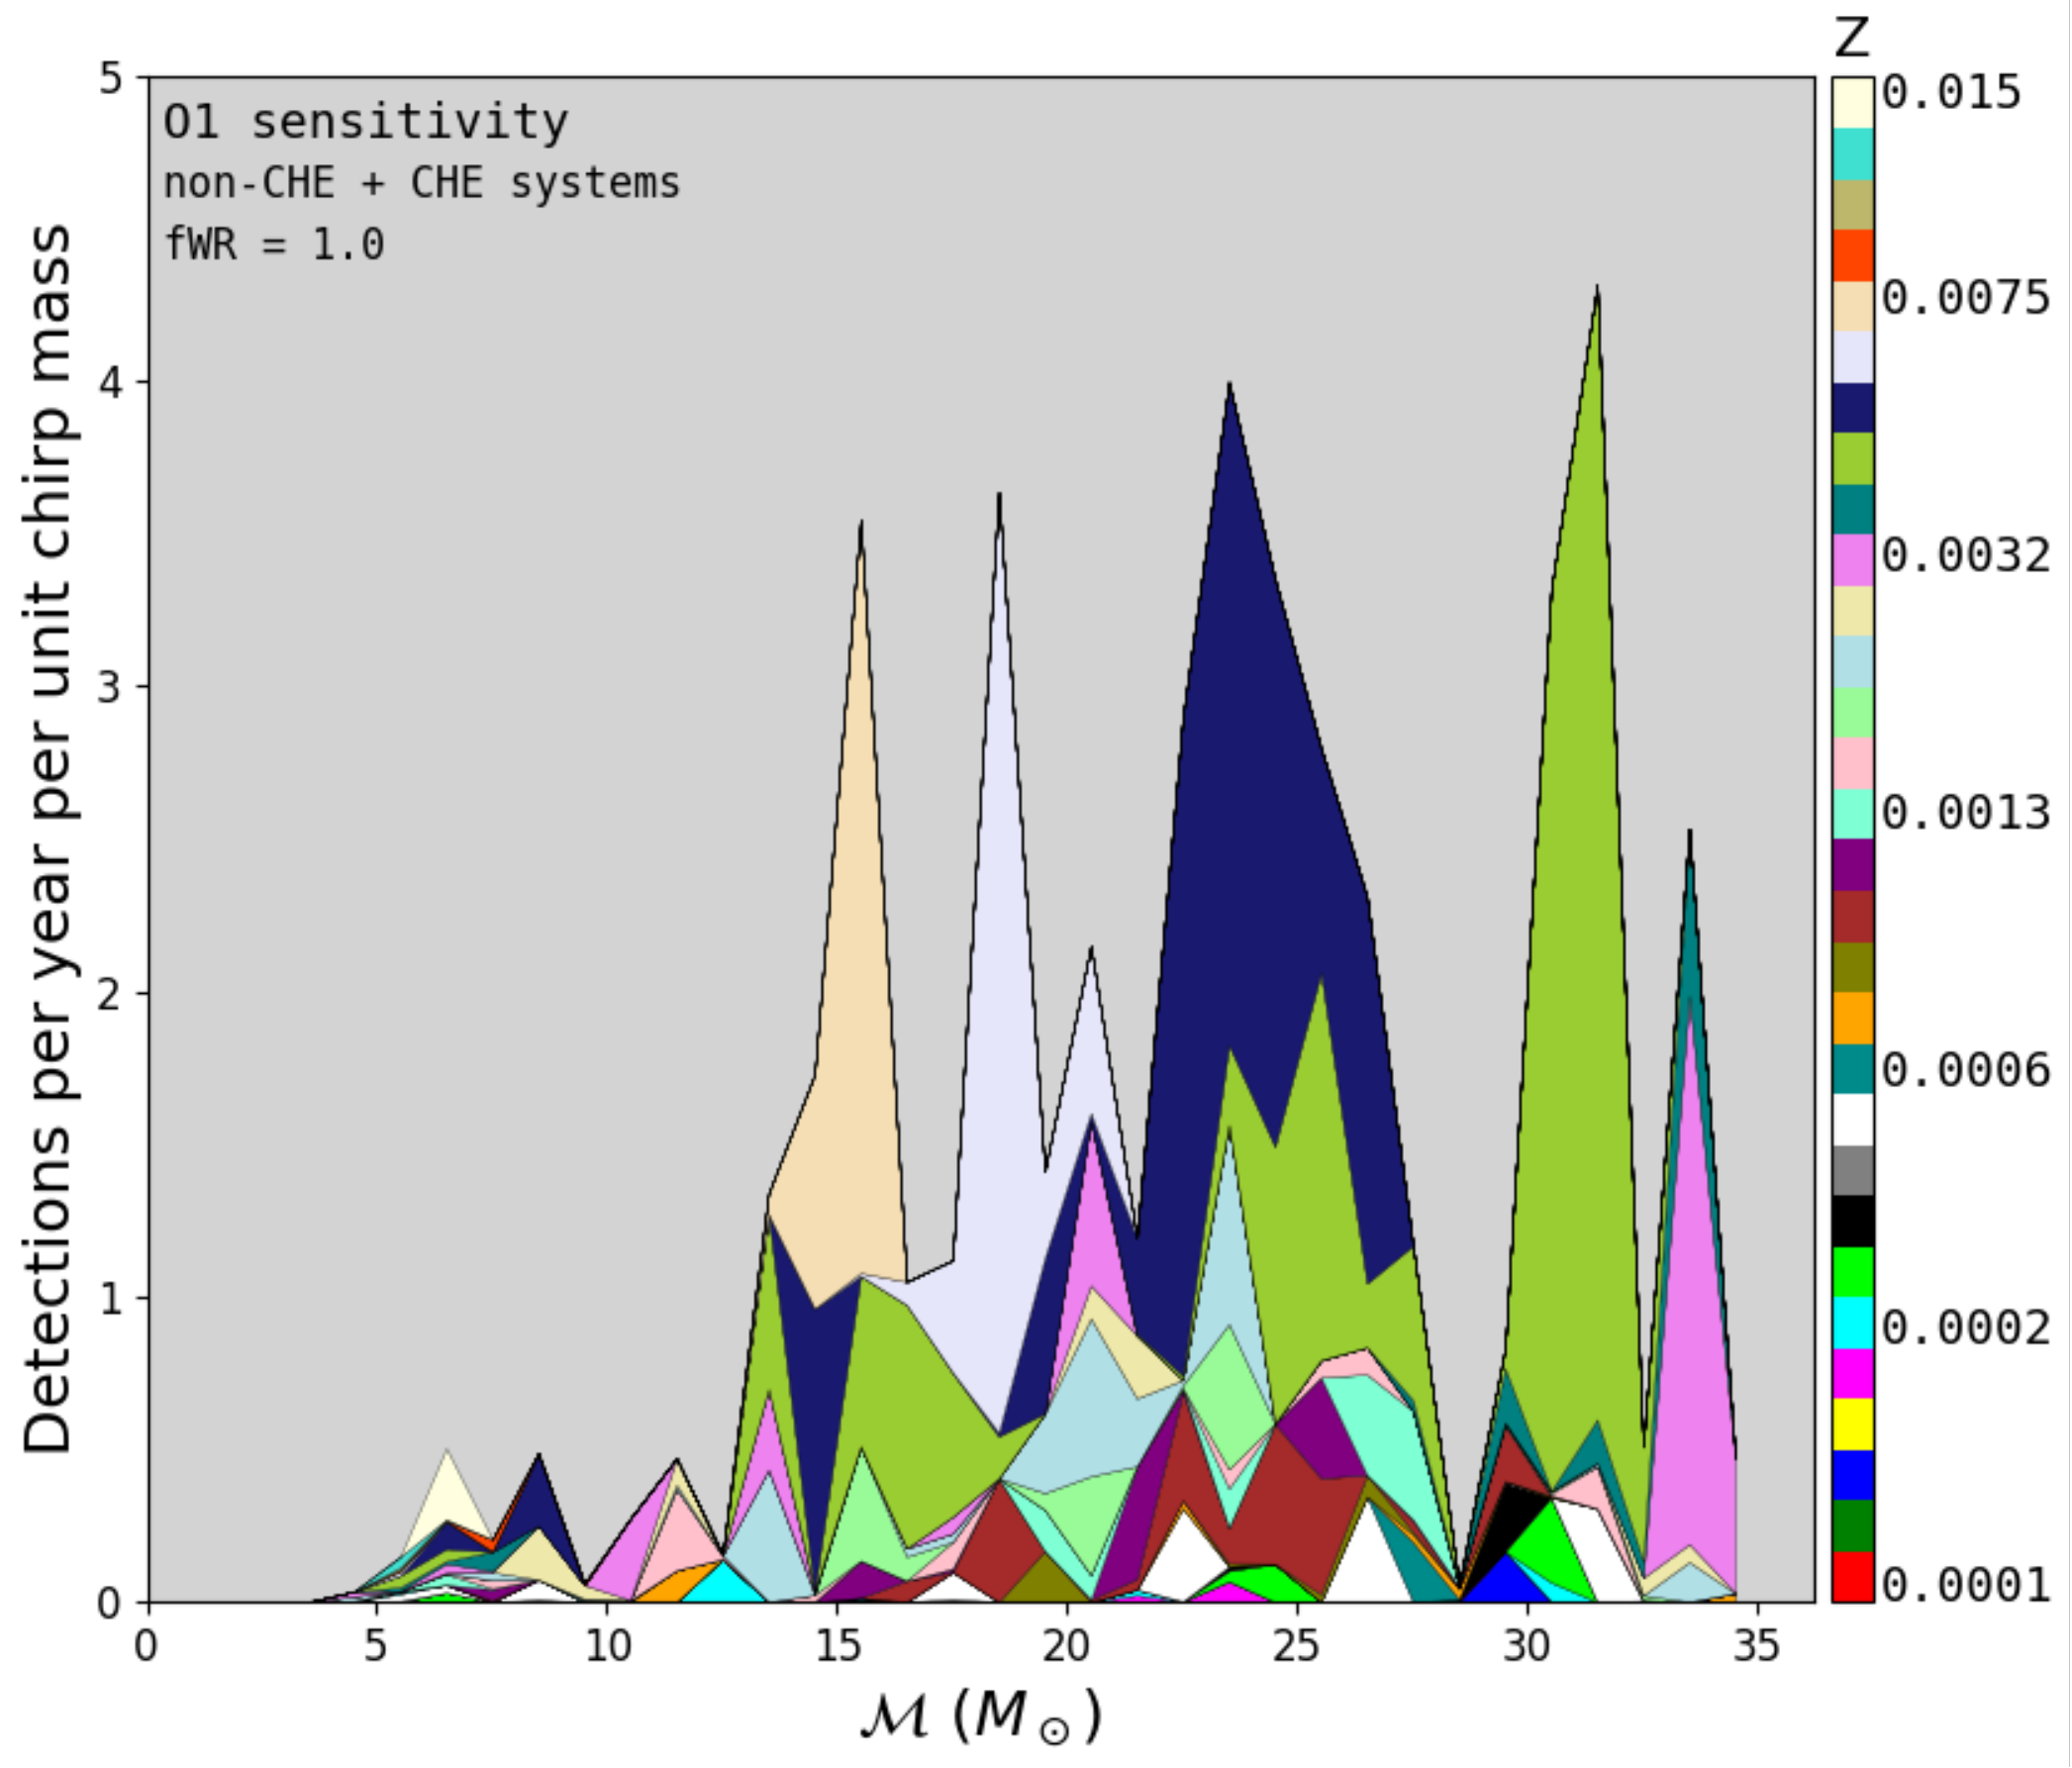}
\captionof{figure}{Predicted chirp mass distribution of \ac{BBH} mergers detectable at aLIGO observing runs 1 and 2 sensitivity for the full population and $f_{wr}=1.0$.  Masses are in the source reference frame.  Colours indicate the contribution of different metallicities.}
\label{fig:Mchirp_O1_fWR1_0_all}

\end{multicols}

Figures~\ref{fig:Mchirp_O1_fWR1_0_che}~and~\ref{fig:Mchirp_O1_fWR1_0_non_che} show the contribution to Figure~\ref{fig:chirp_mass_O1_fWR1_0} of the grid of metallicities for \ac{CHE} systems only (Figure~\ref{fig:Mchirp_O1_fWR1_0_che}), and non-\ac{CHE} systems only (Figure~\ref{fig:Mchirp_O1_fWR1_0_non_che}). Figure~\ref{fig:Mchirp_O1_fWR1_0_che} confirms that the gaps in the \ac{CHE} distribution are not due to the coarseness of the metallicity grid.

\begin{multicols}{2}

\includegraphics[viewport = 5 5 600 510, width=8.45cm, clip]
{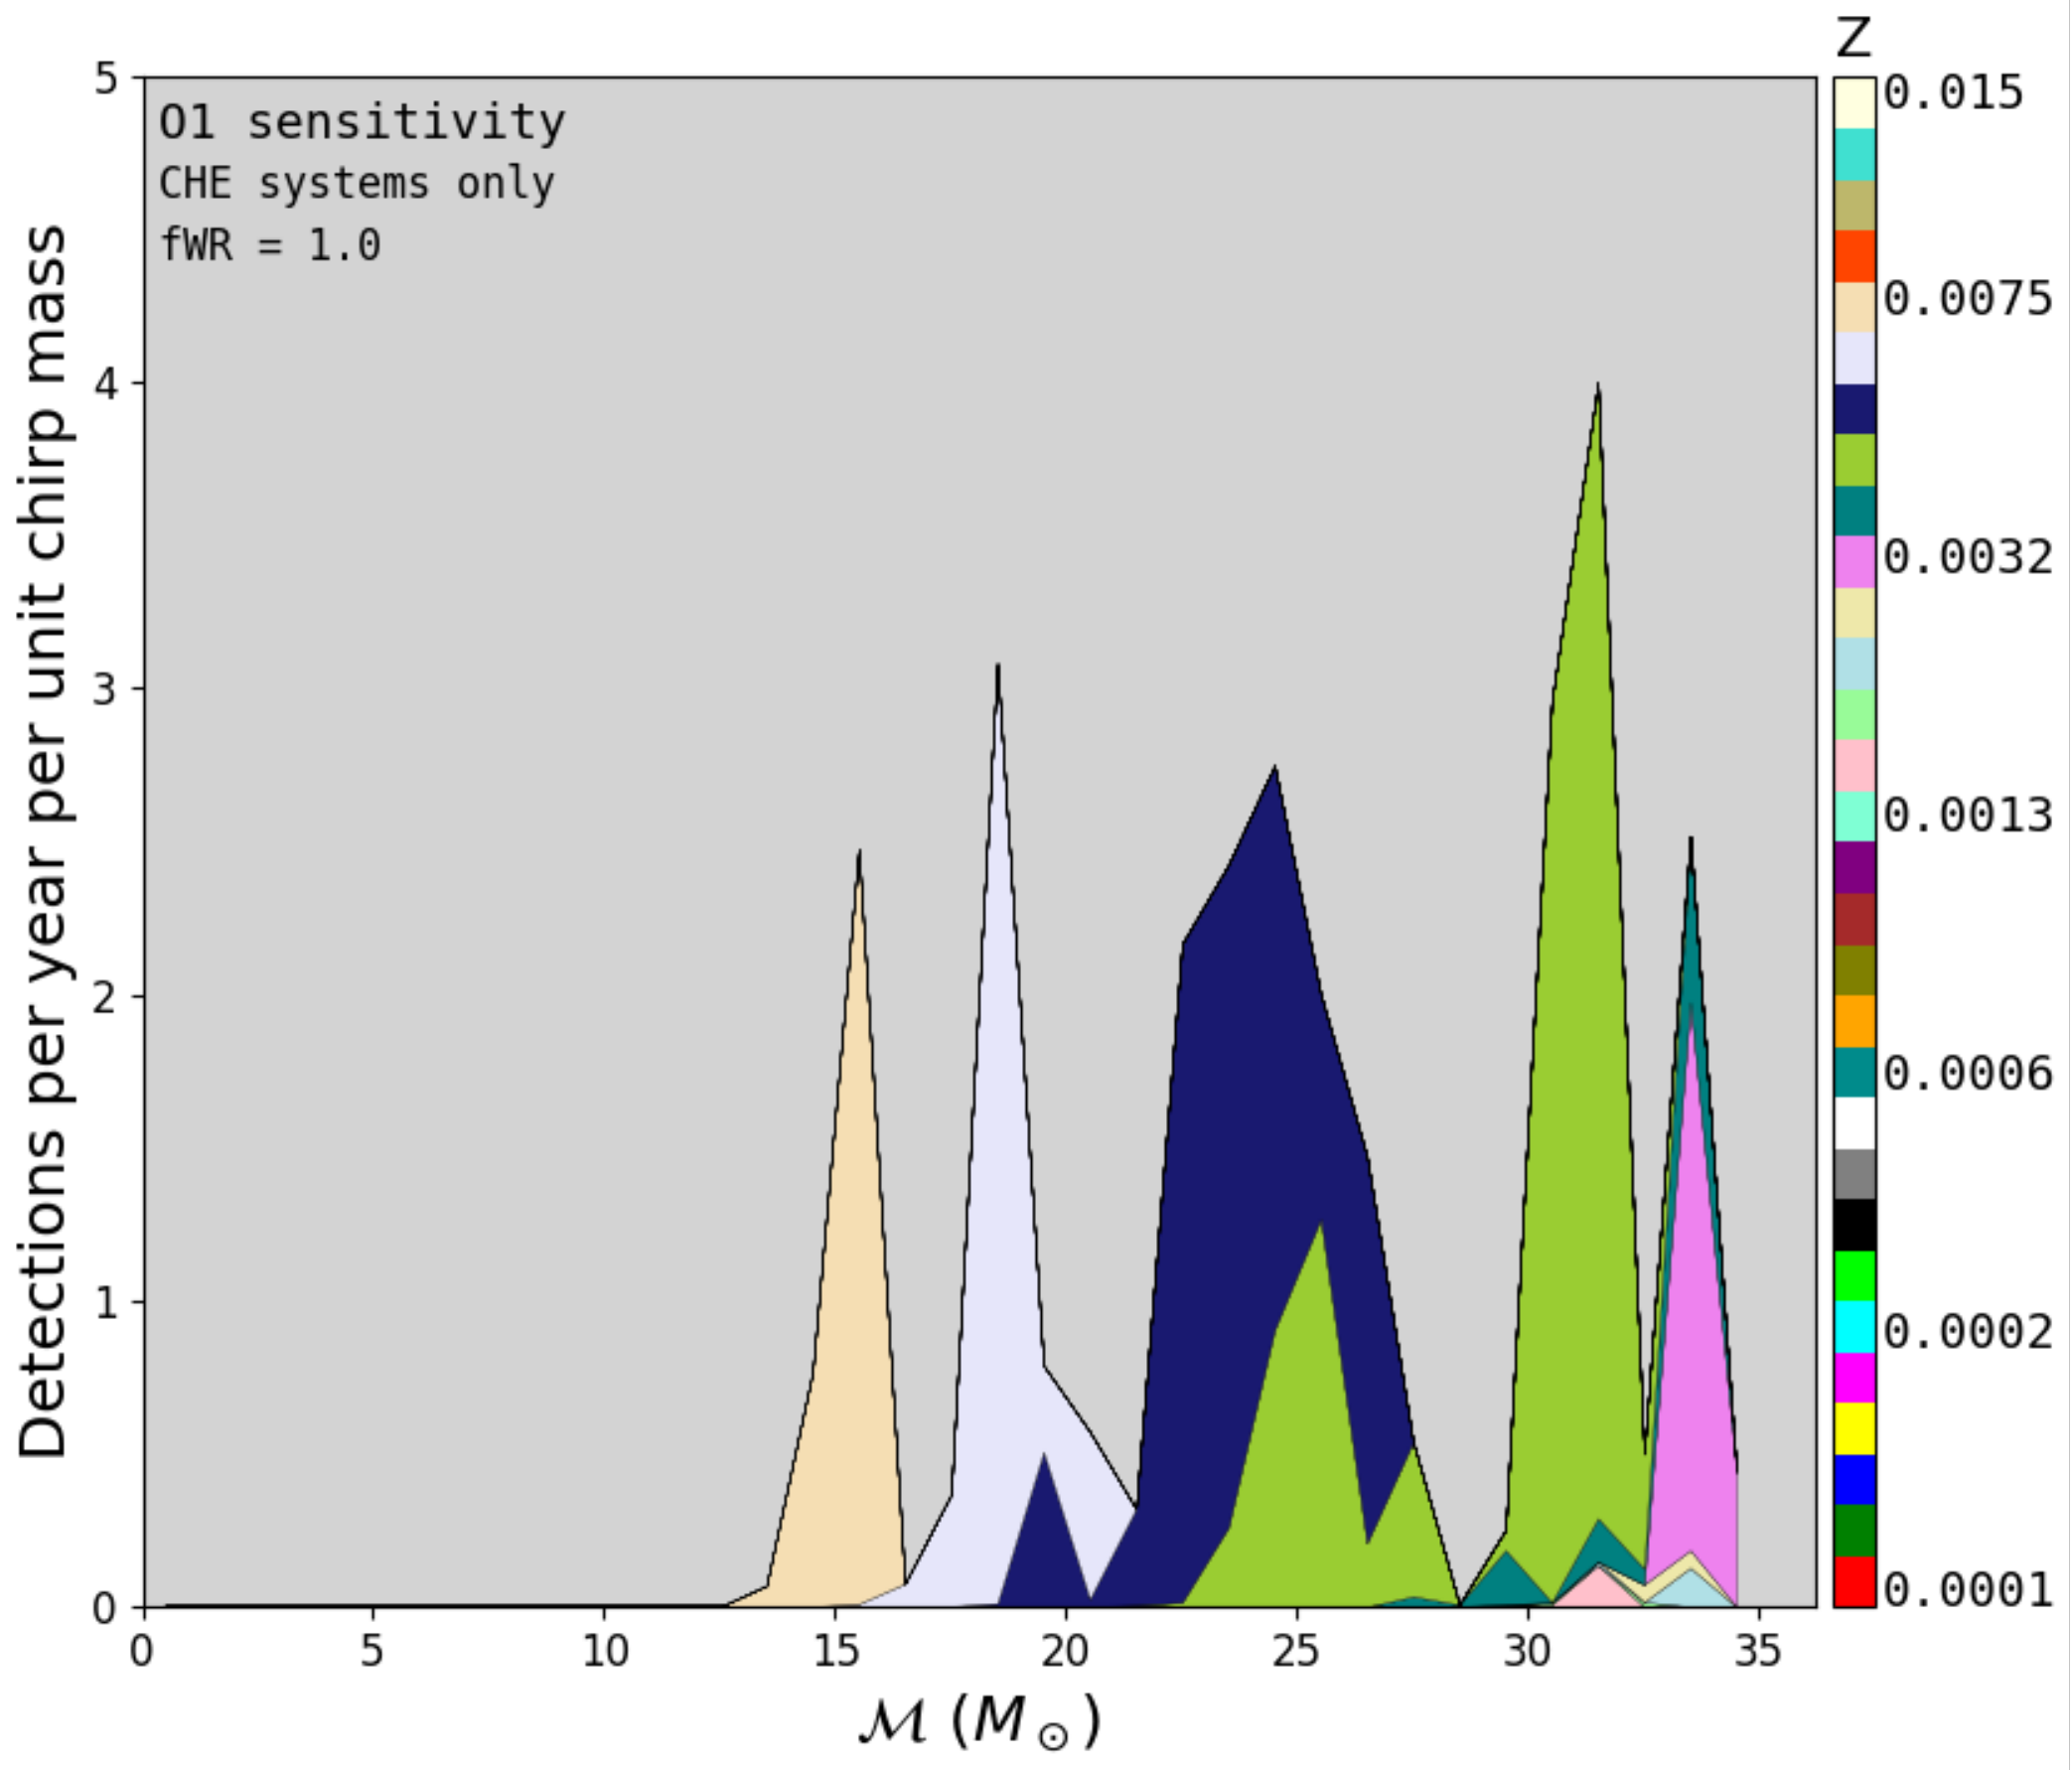}
\captionof{figure}{Predicted chirp mass distribution of \ac{BBH} mergers detectable at aLIGO observing runs 1 and 2 sensitivity for \ac{CHE} systems only and $f_{wr}=1.0$.  Masses are in the source reference frame.  Colours indicate the contribution of different metallicities.}
\label{fig:Mchirp_O1_fWR1_0_che}

\includegraphics[viewport = 5 5 600 510, width=8.45cm, clip]
{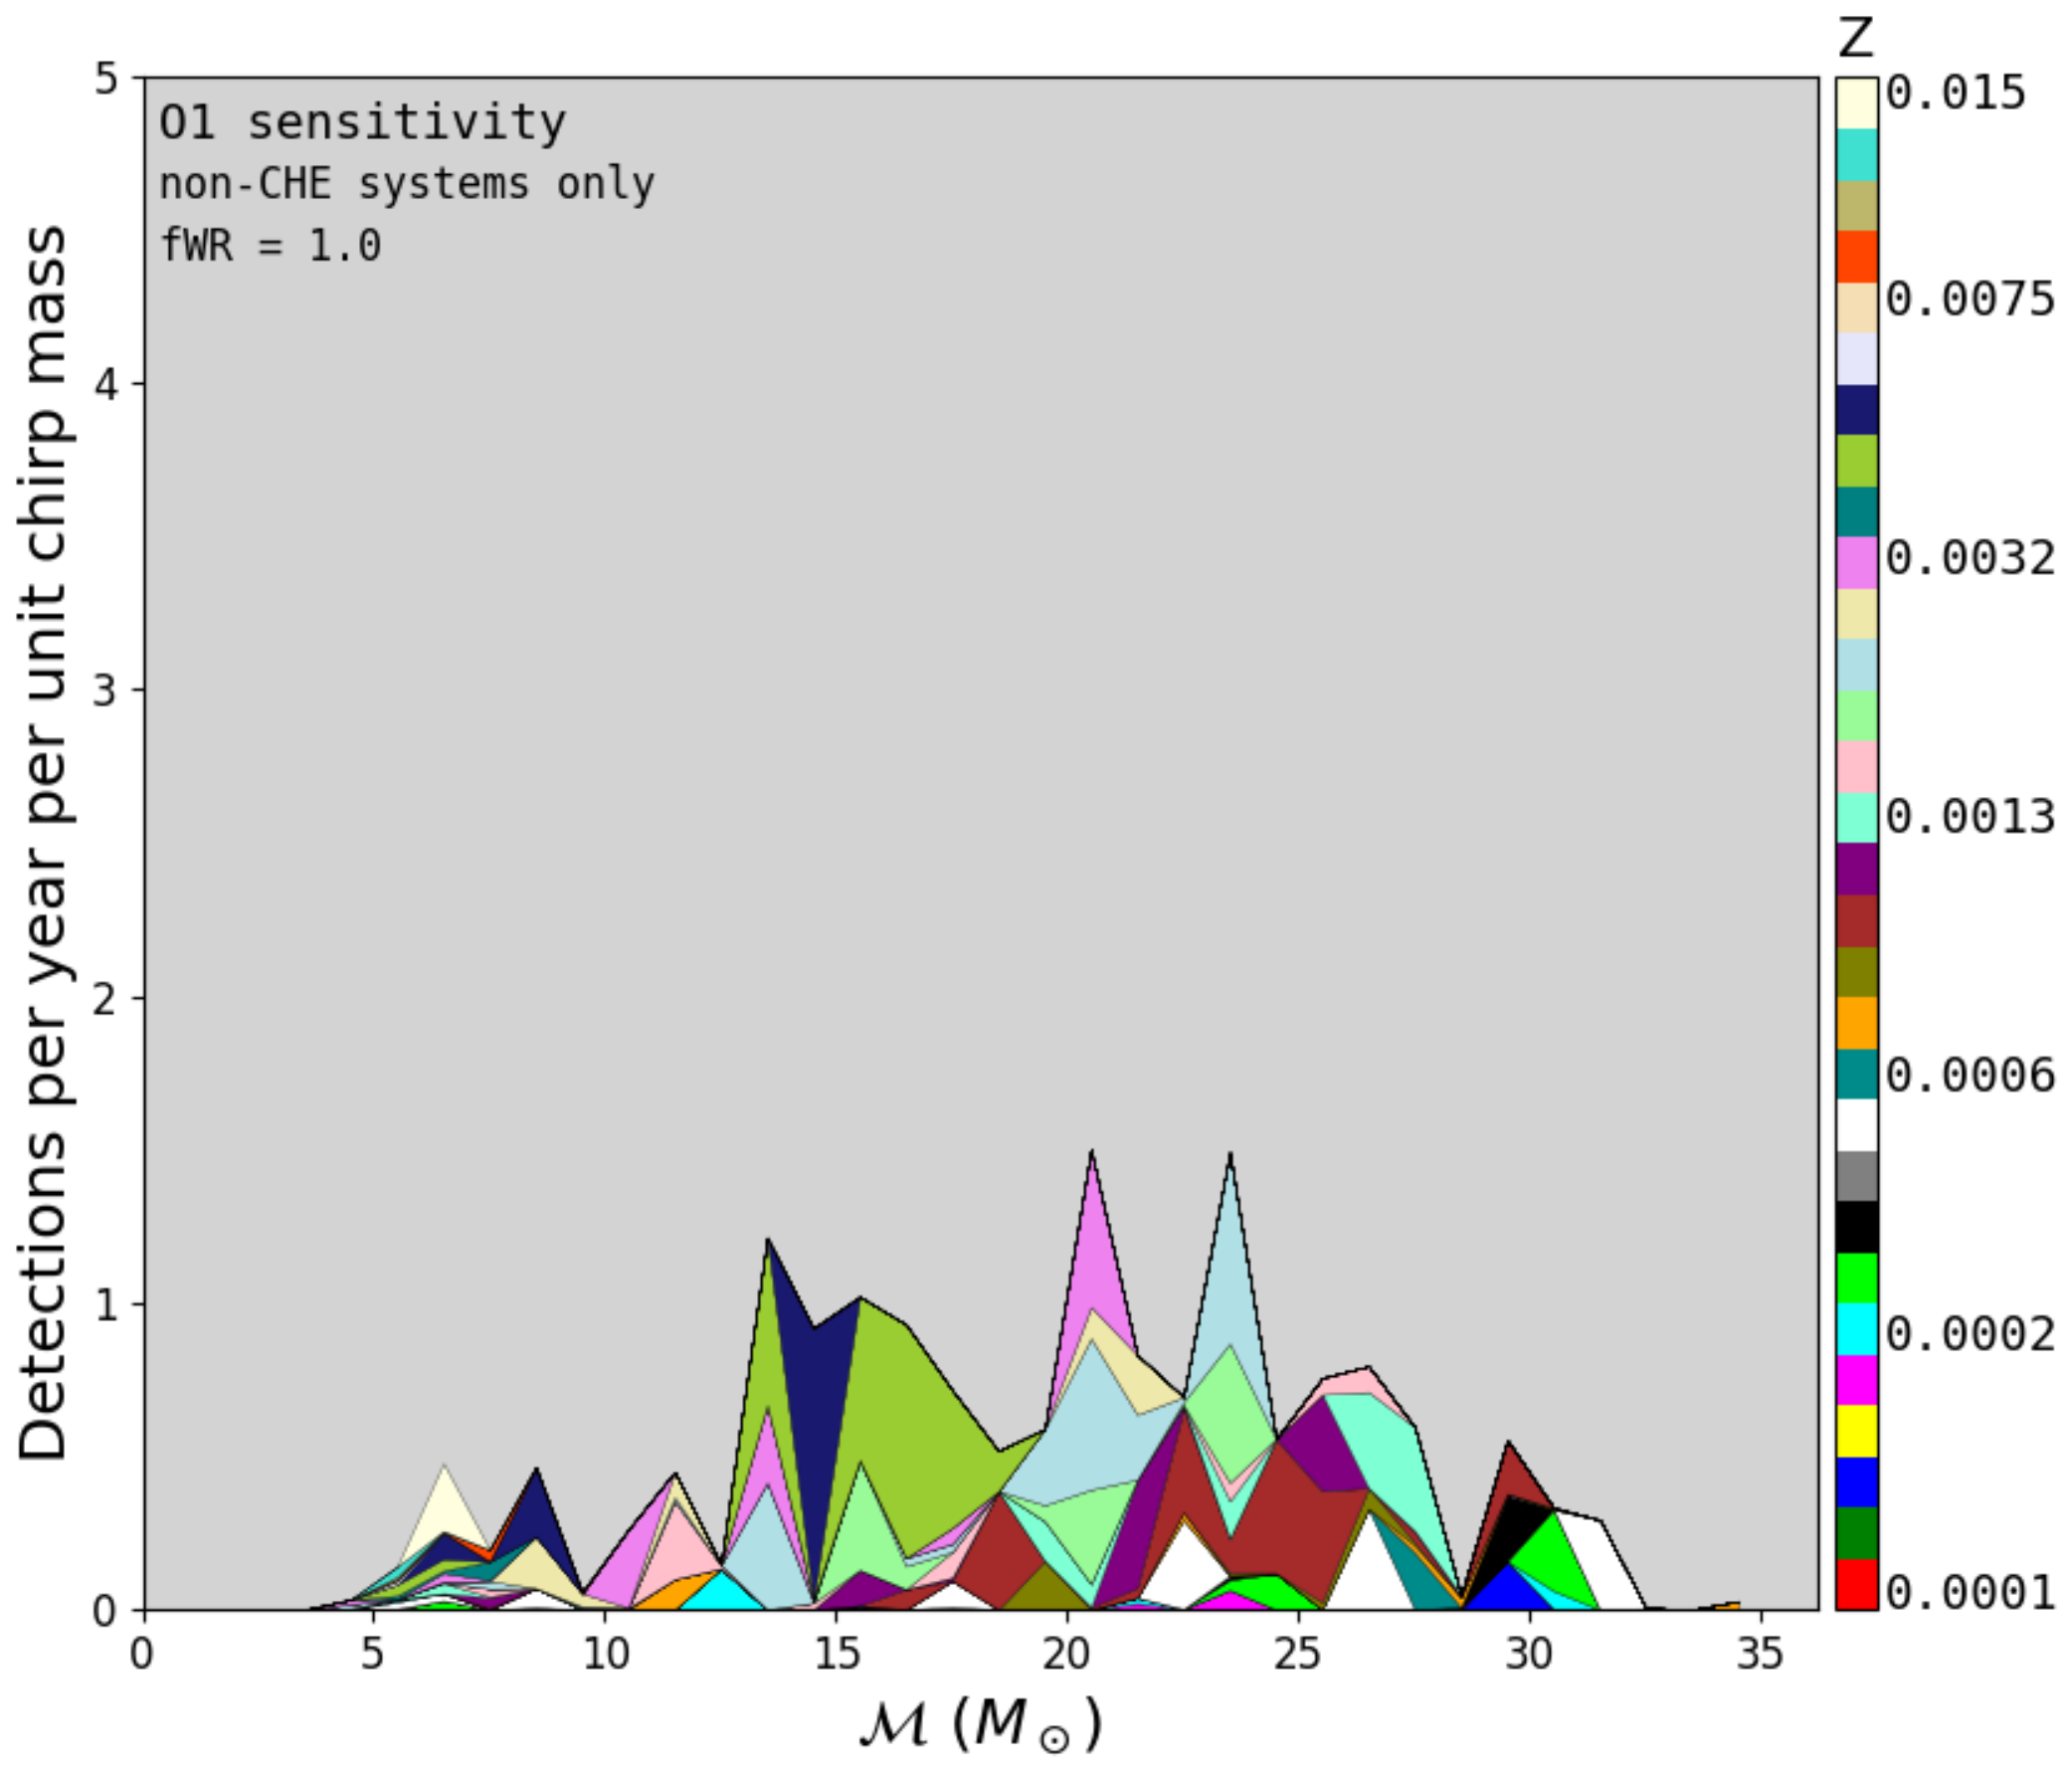}
\captionof{figure}{Predicted chirp mass distribution of \ac{BBH} mergers detectable at aLIGO observing runs 1 and 2 sensitivity for non-\ac{CHE} systems only and $f_{wr}=1.0$.  Masses are in the source reference frame.  Colours indicate the contribution of different metallicities.}
\label{fig:Mchirp_O1_fWR1_0_non_che}

\end{multicols}

\begin{multicols}{2}

As stated in Section~\ref{sec:results}, we evolved $12$ million binary systems: $100,000$ for each of the $120$ combinations of $Z$ and $f_{wr}$. Figure~\ref{fig:Mchirp_O1_fWr1_0_Z-2_35_che} shows the \ac{CHE} distribution for the population of 100,000 systems evolved for $f_{wr}=1.0$ and $log_{10}(Z)=-2.35$. We evolved a further 1,000,000 binary systems for $f_{wr}=1.0$ and $log_{10}(Z)=-2.35$: the \ac{CHE} distribution for that population is shown in Figure~\ref{fig:Mchirp_O1_fWR1_0_Z-2_35_fullPop}. It is clear from Figures~\ref{fig:Mchirp_O1_fWr1_0_Z-2_35_che}~and~\ref{fig:Mchirp_O1_fWR1_0_Z-2_35_fullPop} that the gaps in the \ac{CHE} \ac{PDF} are due to the relatively low number of \ac{BBH} mergers in our original population of 100,000 systems that are detectable at \ac{aLIGO} observing runs 1 and 2 sensitivity, and that the distribution is described more completely by sampling more binary systems in the corresponding parameter space.

\end{multicols}

\begin{multicols}{2}

\includegraphics[viewport = 5 3 555 510, width=8.45cm, clip]
{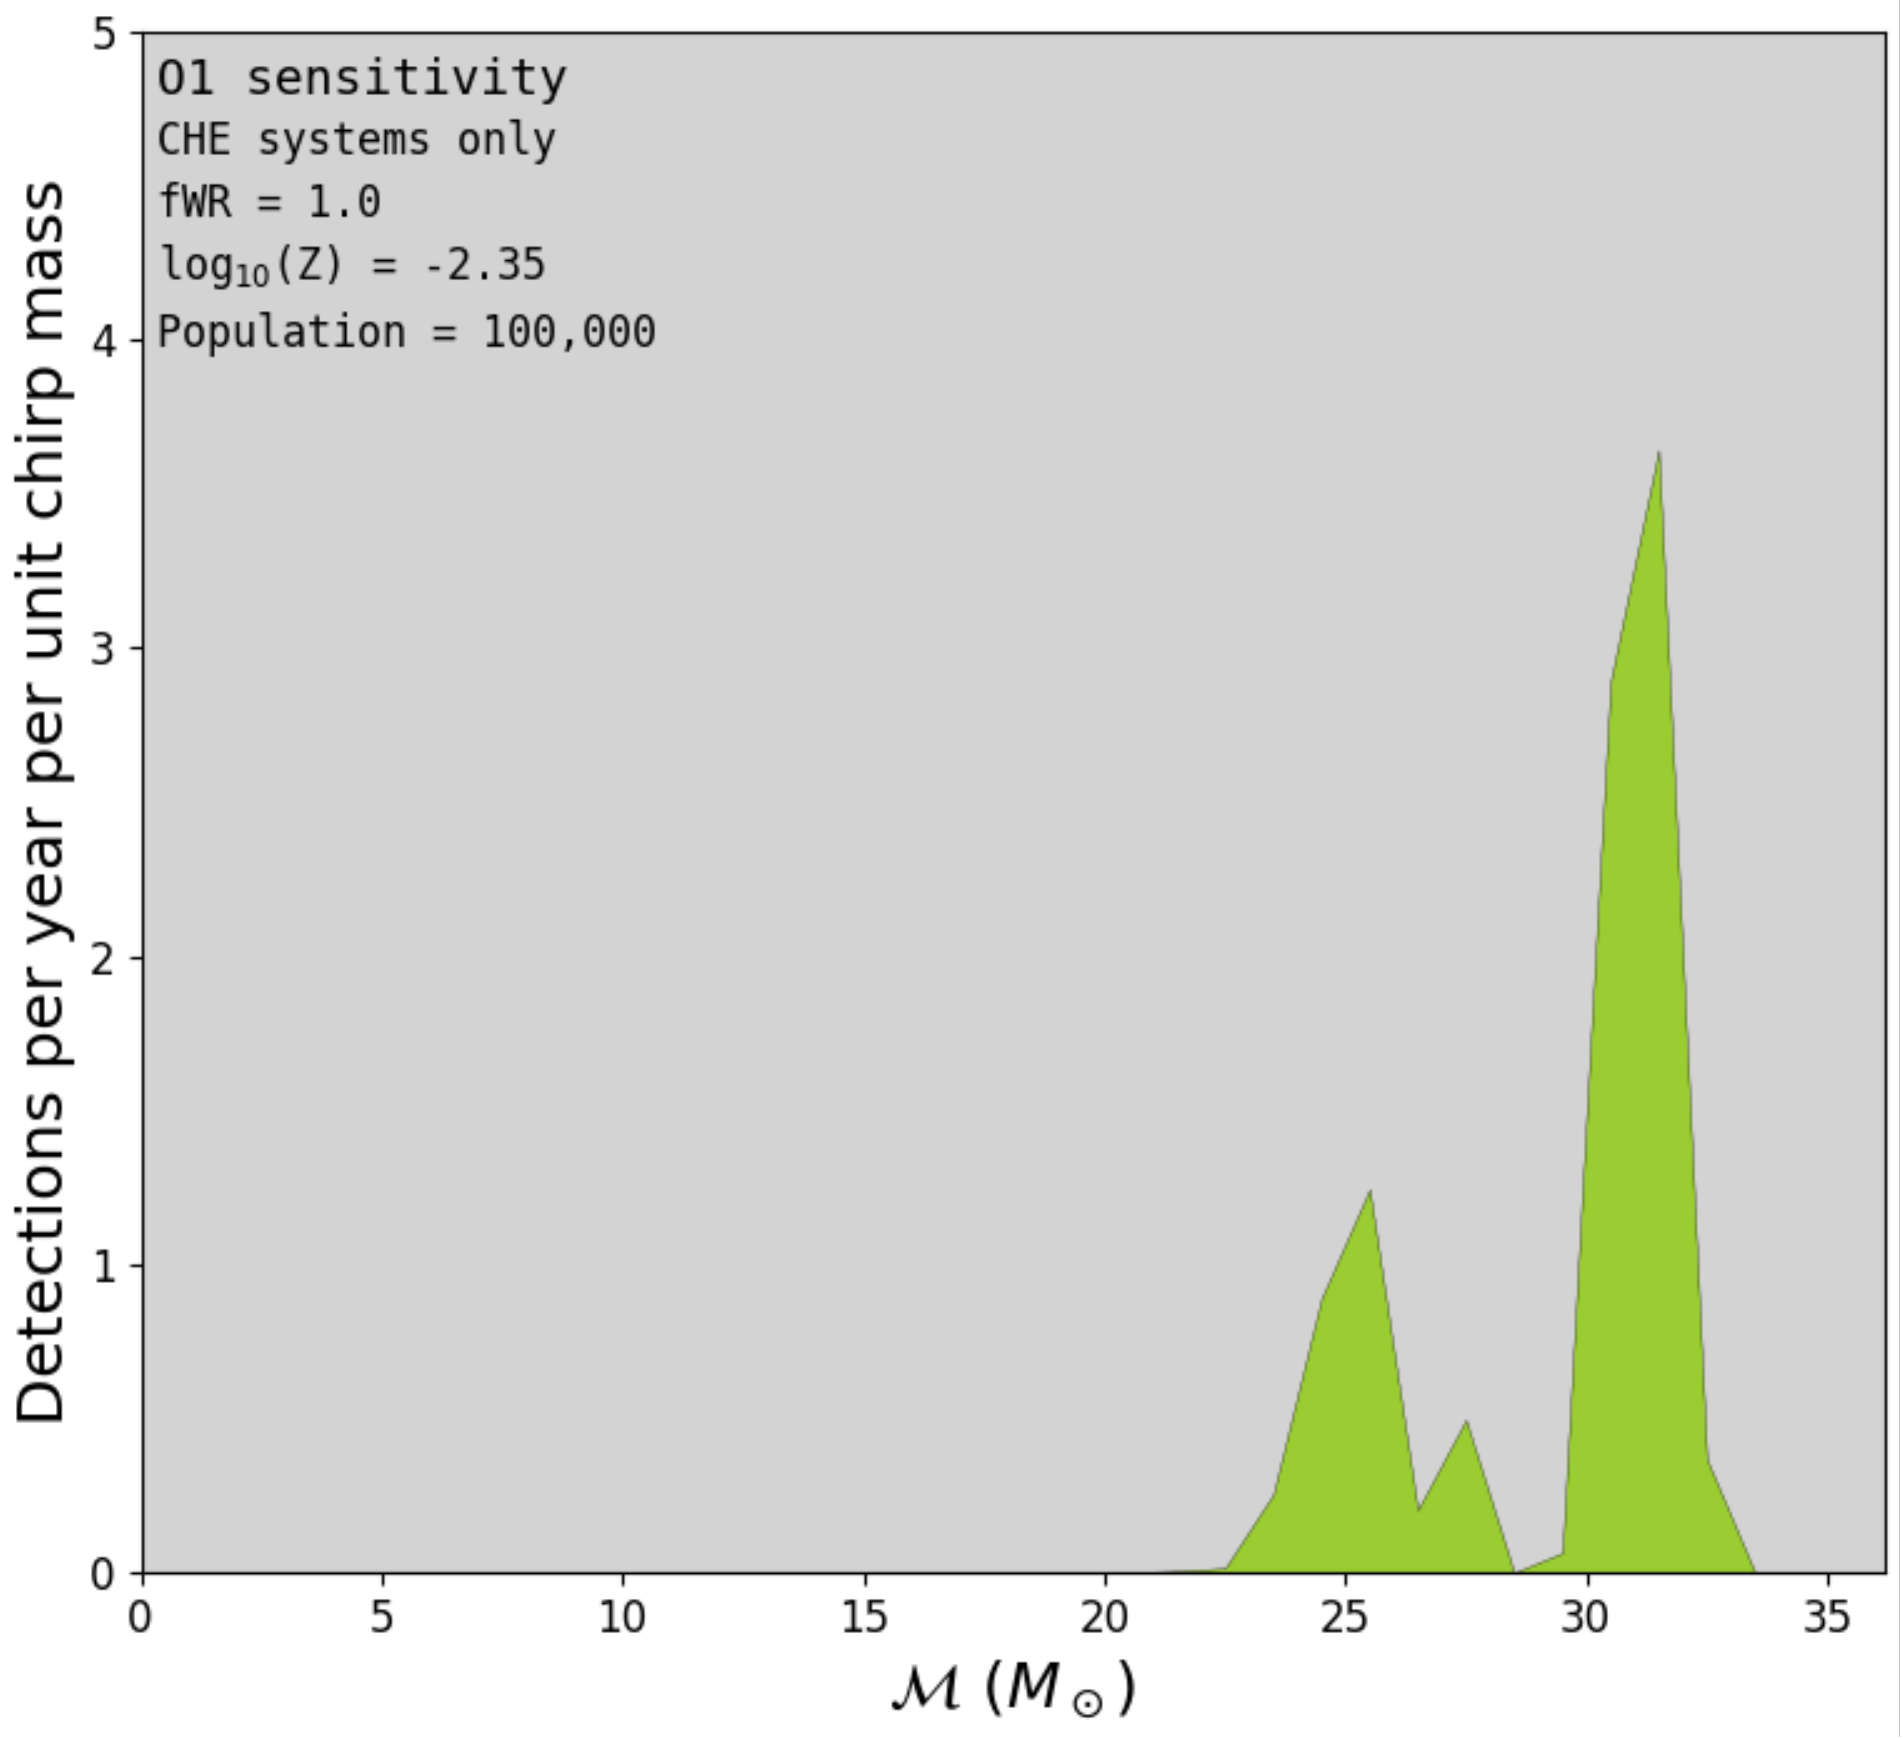}
\captionof{figure}{Predicted chirp mass distribution of \ac{BBH} mergers detectable at aLIGO observing runs 1 and 2 sensitivity for \ac{CHE} systems only from the initial population of 100,000 simulations with $f_{wr}=1.0$ and $log_{10}(Z)=-2.35$.  Masses are in the source reference frame.}
\label{fig:Mchirp_O1_fWr1_0_Z-2_35_che}

\includegraphics[viewport = 5 3 555 510, width=8.45cm, clip]
{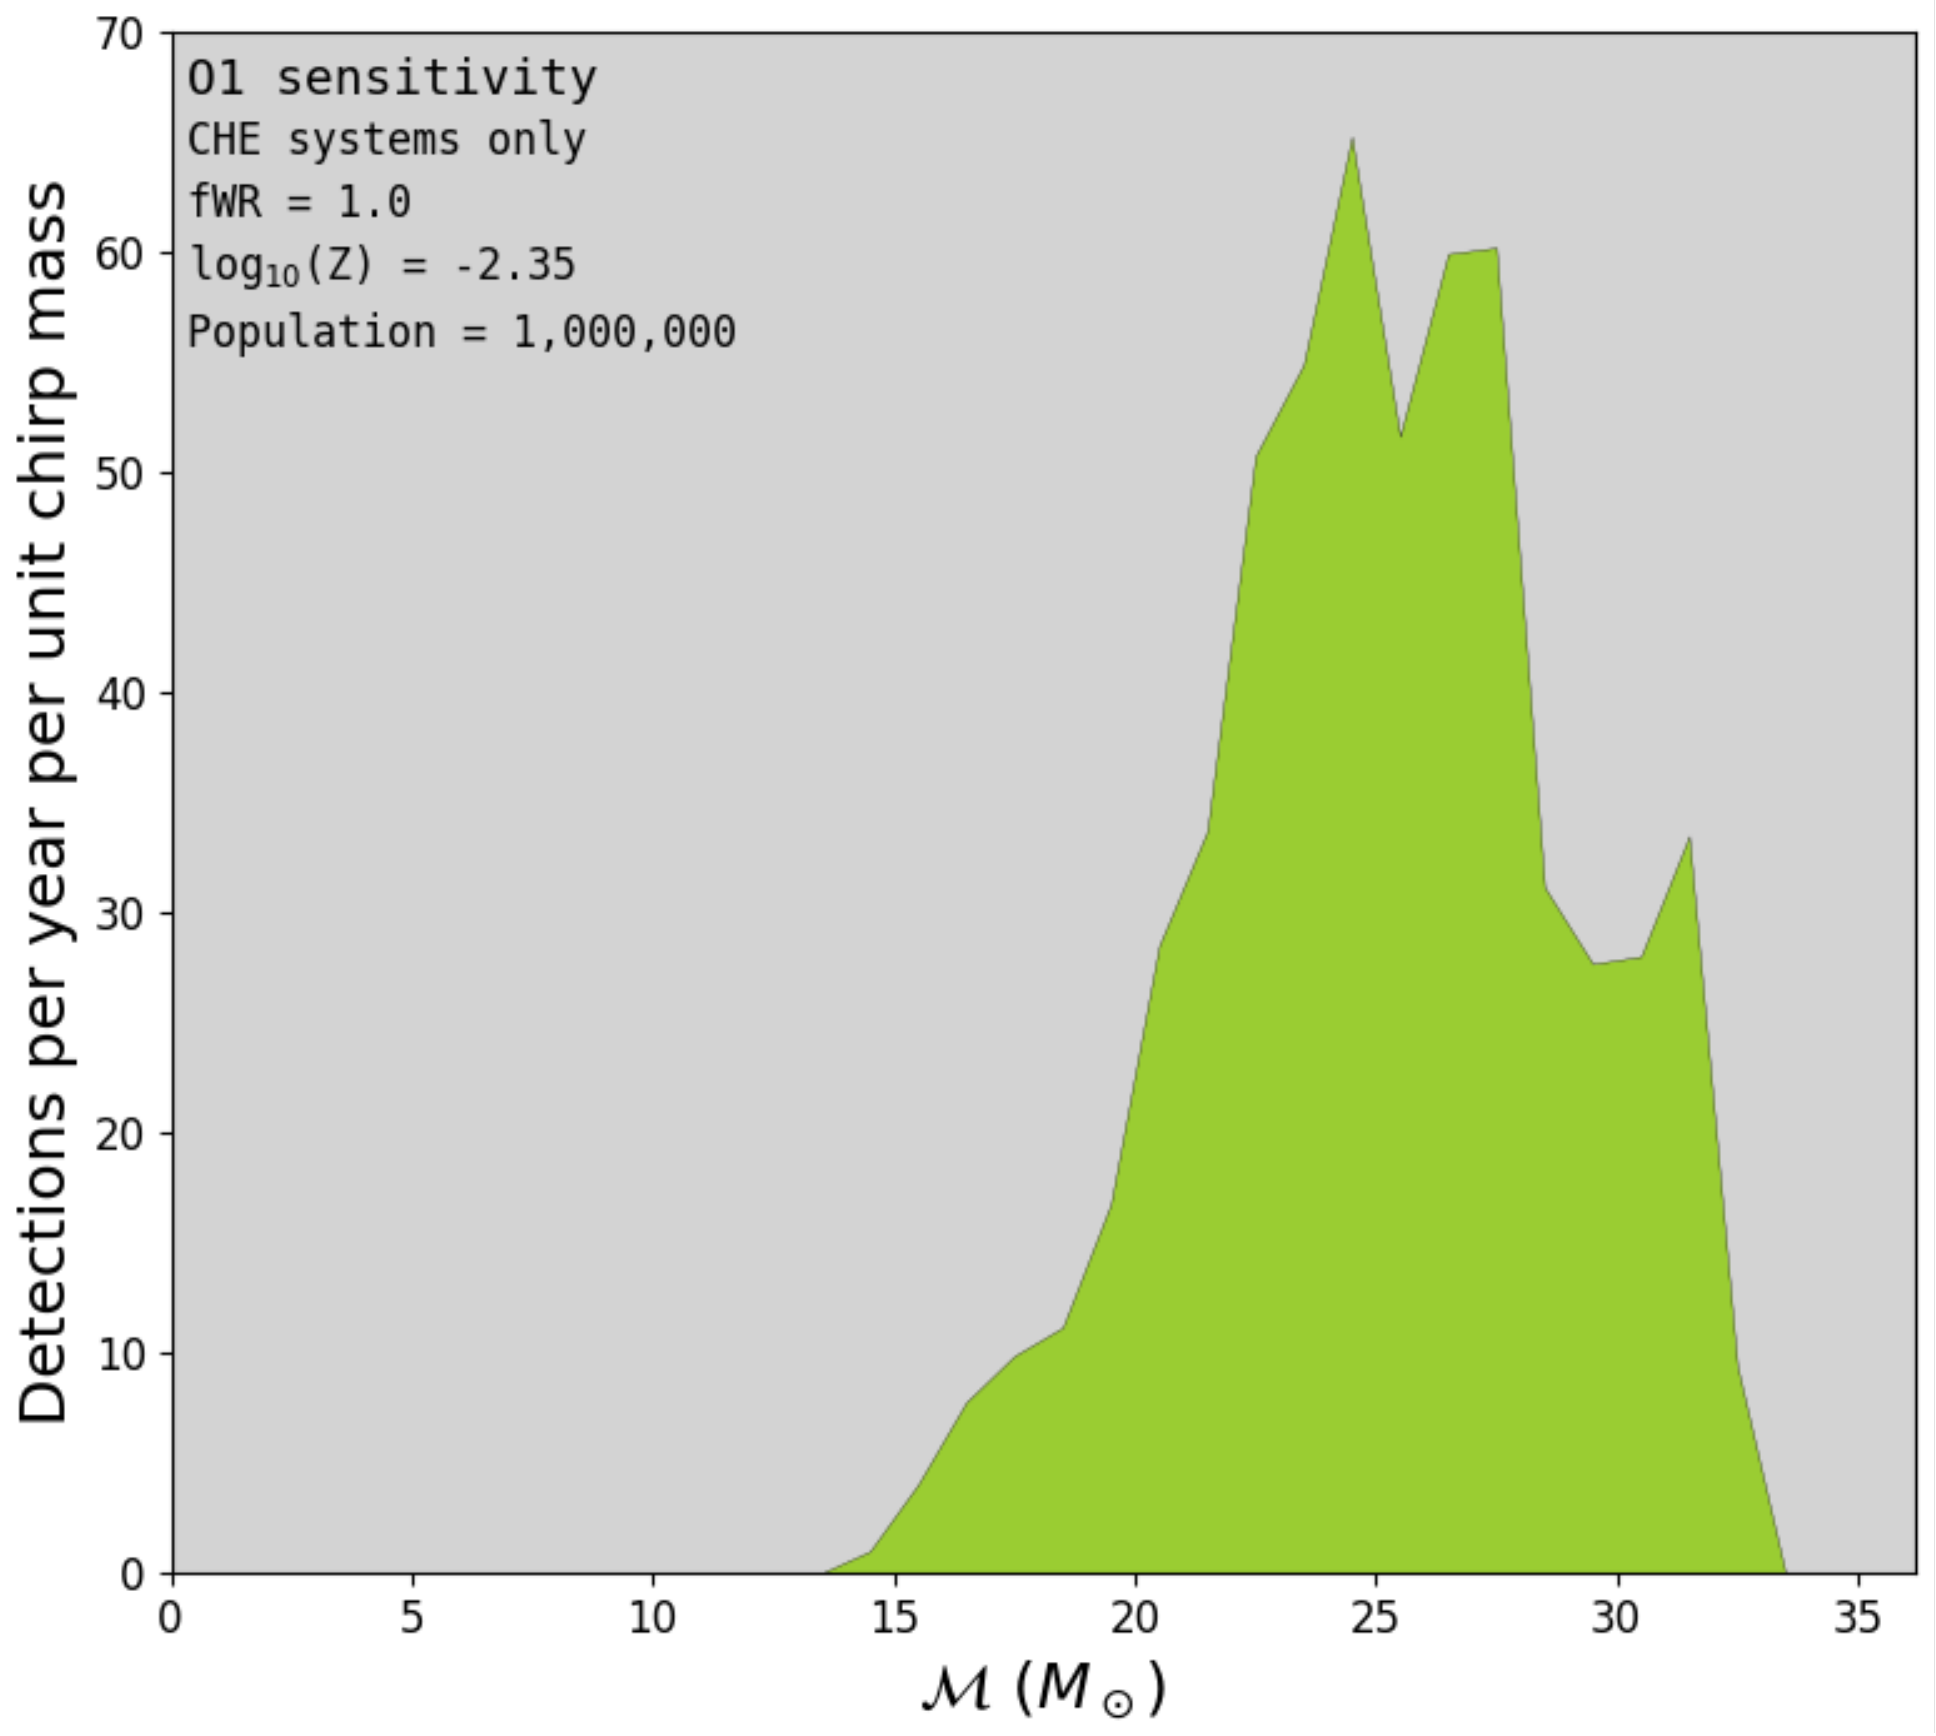}
\captionof{figure}{Predicted chirp mass distribution of \ac{BBH} mergers detectable at aLIGO observing runs 1 and 2 sensitivity for \ac{CHE} systems only from the additional population of 1,000,000 simulations with $f_{wr}=1.0$ and $log_{10}(Z)=-2.35$.  Masses are in the source reference frame.}
\label{fig:Mchirp_O1_fWR1_0_Z-2_35_fullPop}

\end{multicols}
