# Supplementary material for: Chemically Homogeneous Evolution: A rapid population synthesis approach
Source: arXiv:2010.00002 source file (2021-05-02)
Supplement: Supplementary file 2 [file appendix-PeriodVsMassPlots.tex]

\onecolumn
\begin{multicols}{2}
\section{Period vs mass plots}\label{sec:pFinalVSmTotal_individual_WR_plots}
\ilya{[Do we need this appendix / these plots? What are they telling us that we haven't already seen?]}

\jeff{[Probably not.  I put them in because I had them and they provide a little more clarity and detail than the combined plot - just because they are not overlaid. Happy to remove the appendix if you don't think it should be included.]}
\subsection{Initial attributes}\label{subsec:pInitialVSmTotal_plots}

Figures~\ref{fig:pInitialVSmTotal_fWR0_0}, \ref{fig:pInitialVSmTotal_fWR0_2}, \ref{fig:pInitialVSmTotal_fWR0_6}, and ~\ref{fig:pInitialVSmTotal_fWR1_0} show initial system total masses and orbital periods for \ac{CHE} systems that have formed \acp{BBH} that will merge within 14 Gyr for \ac{WR} wind factors $0.0,\ 0.2,\ 0.6,$ and $1.0$ respectively. These are the constituent plots that, when overlaid, make up Figure~\ref{fig:pInitialVSmTotal_fWRall}.

See Section~\ref{subsec:pop_synth} for a detailed description of these plots.

\end{multicols}

% forcing placement of the plots by not wrapping it in /begin{figure}.../end{figure}
\begin{multicols}{2}

\includegraphics[width=0.475\textwidth]{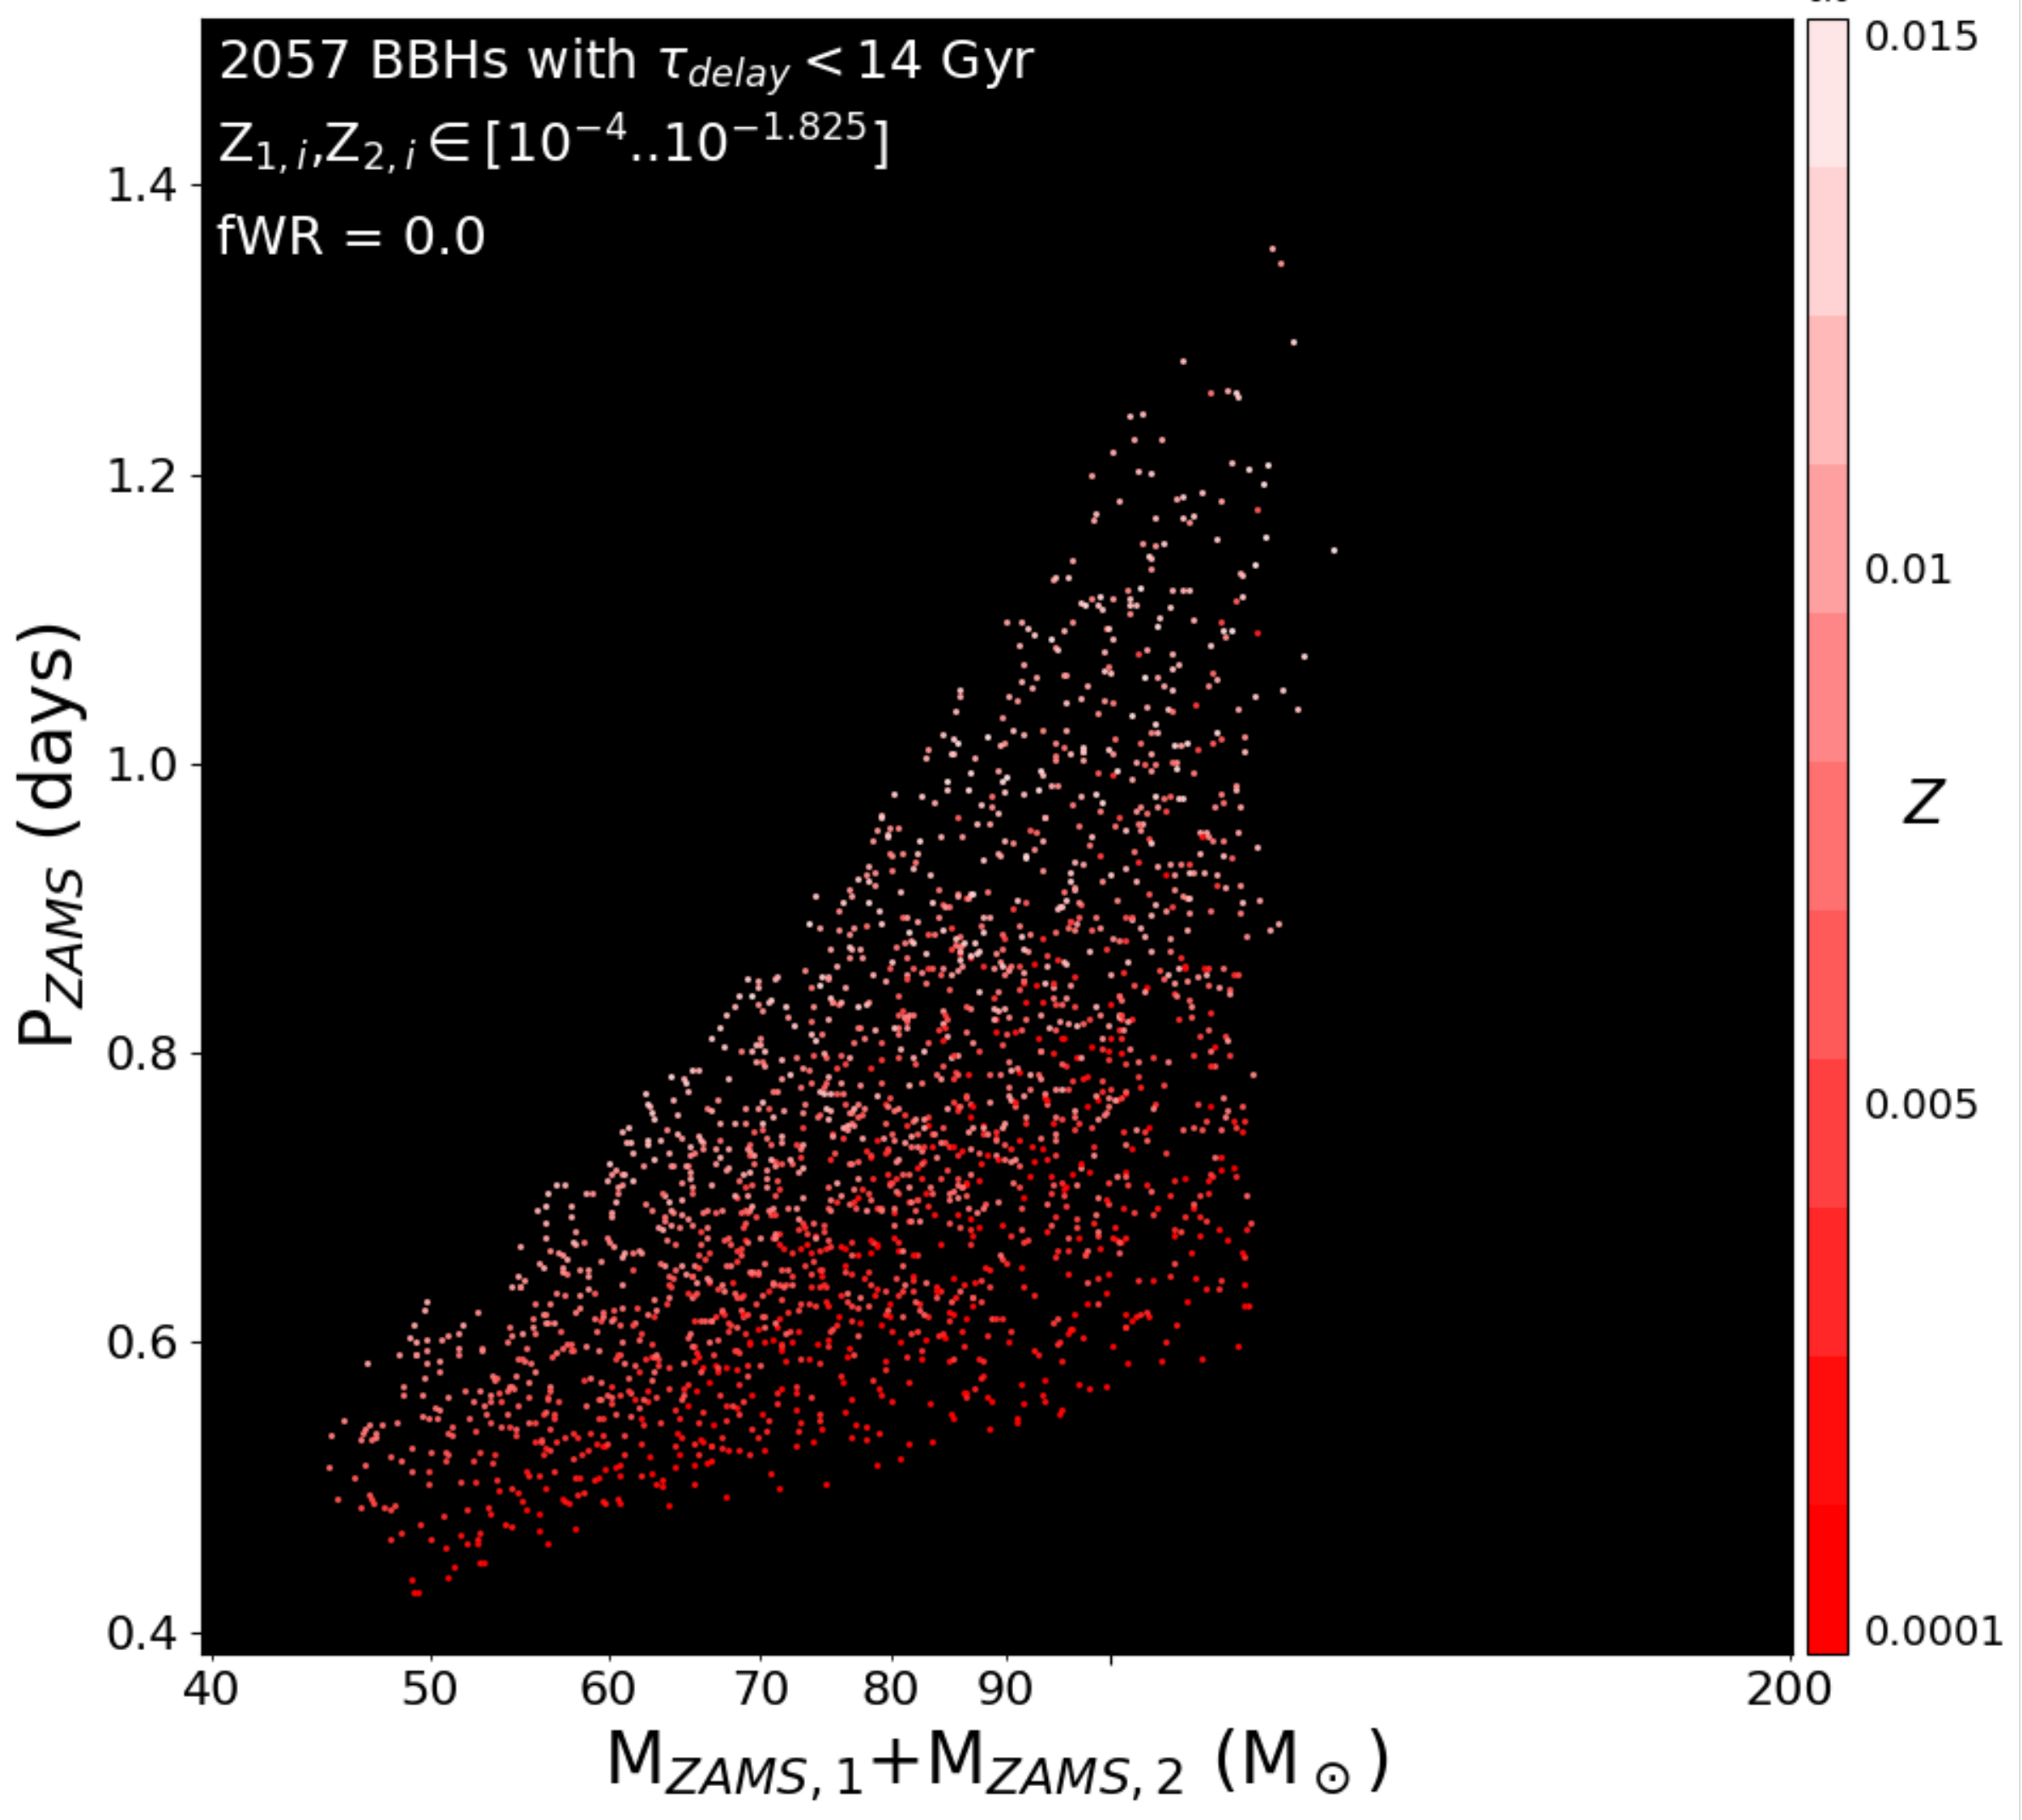}
\captionof{figure}{$f_{wr}=0.0$}
\label{fig:pInitialVSmTotal_fWR0_0}

\includegraphics[width=0.475\textwidth]{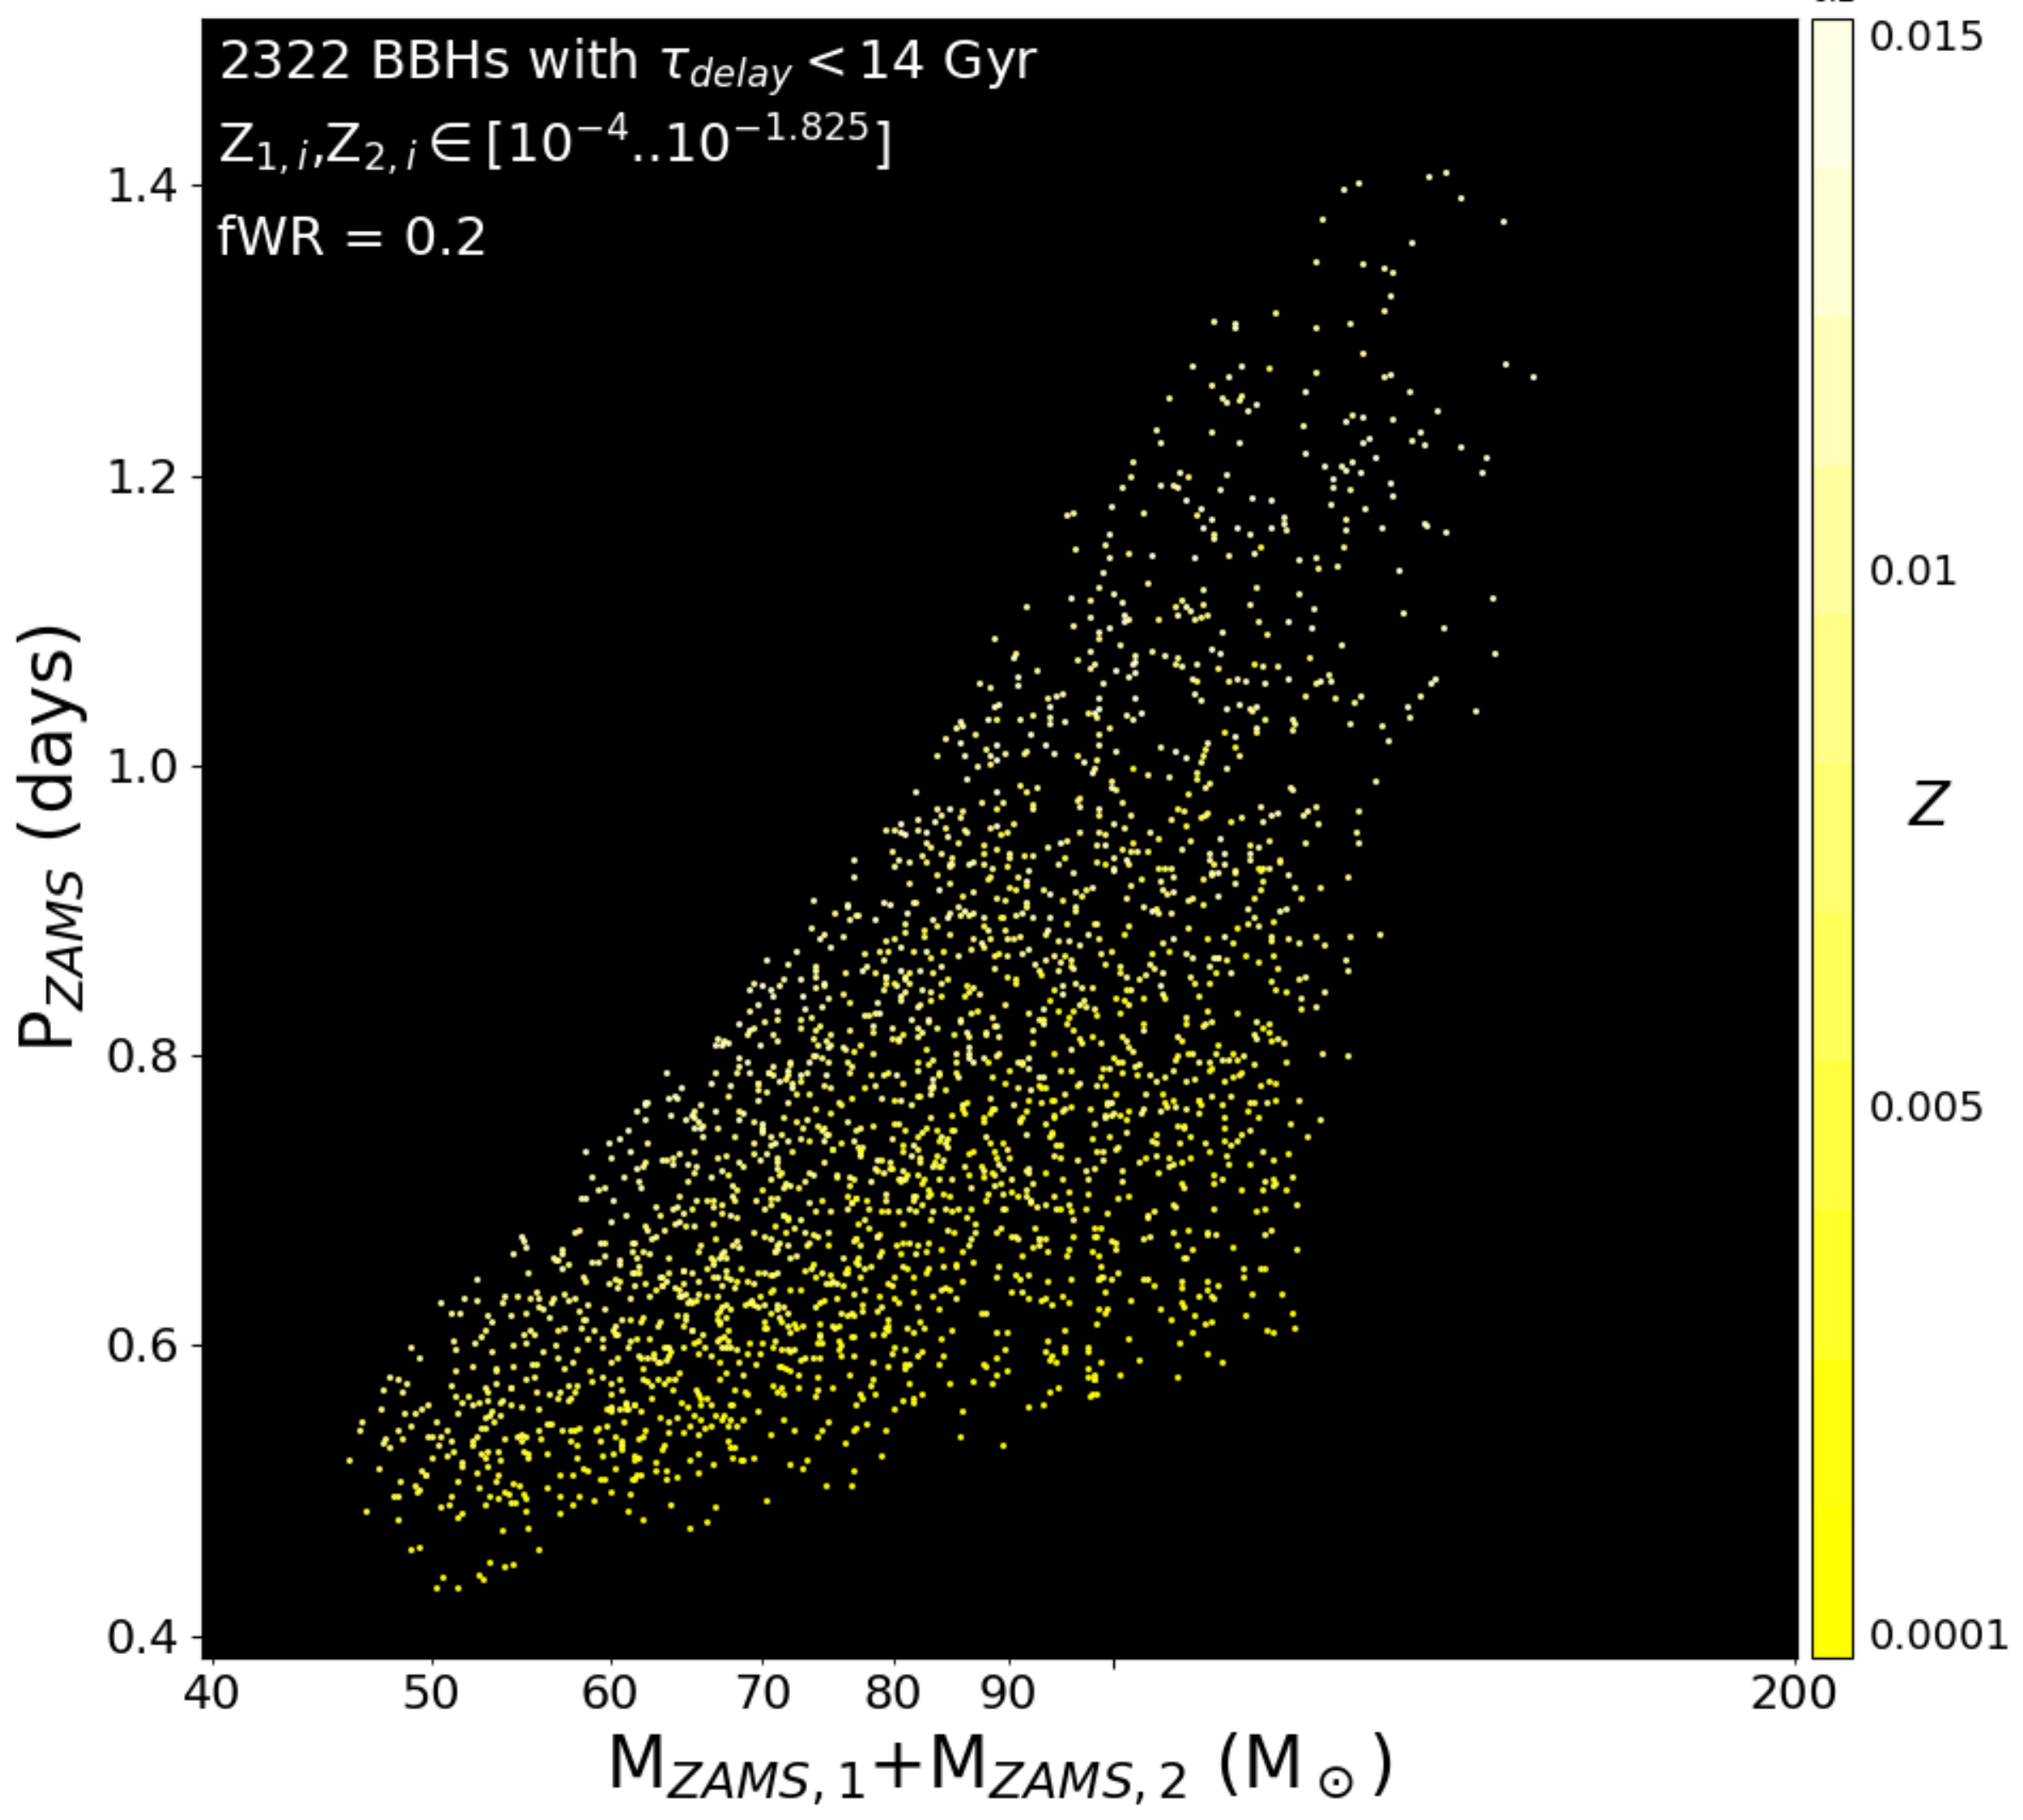}
\captionof{figure}{$f_{wr}=0.2$}
\label{fig:pInitialVSmTotal_fWR0_2}

\end{multicols}
\begin{multicols}{2}

\includegraphics[width=0.475\textwidth]{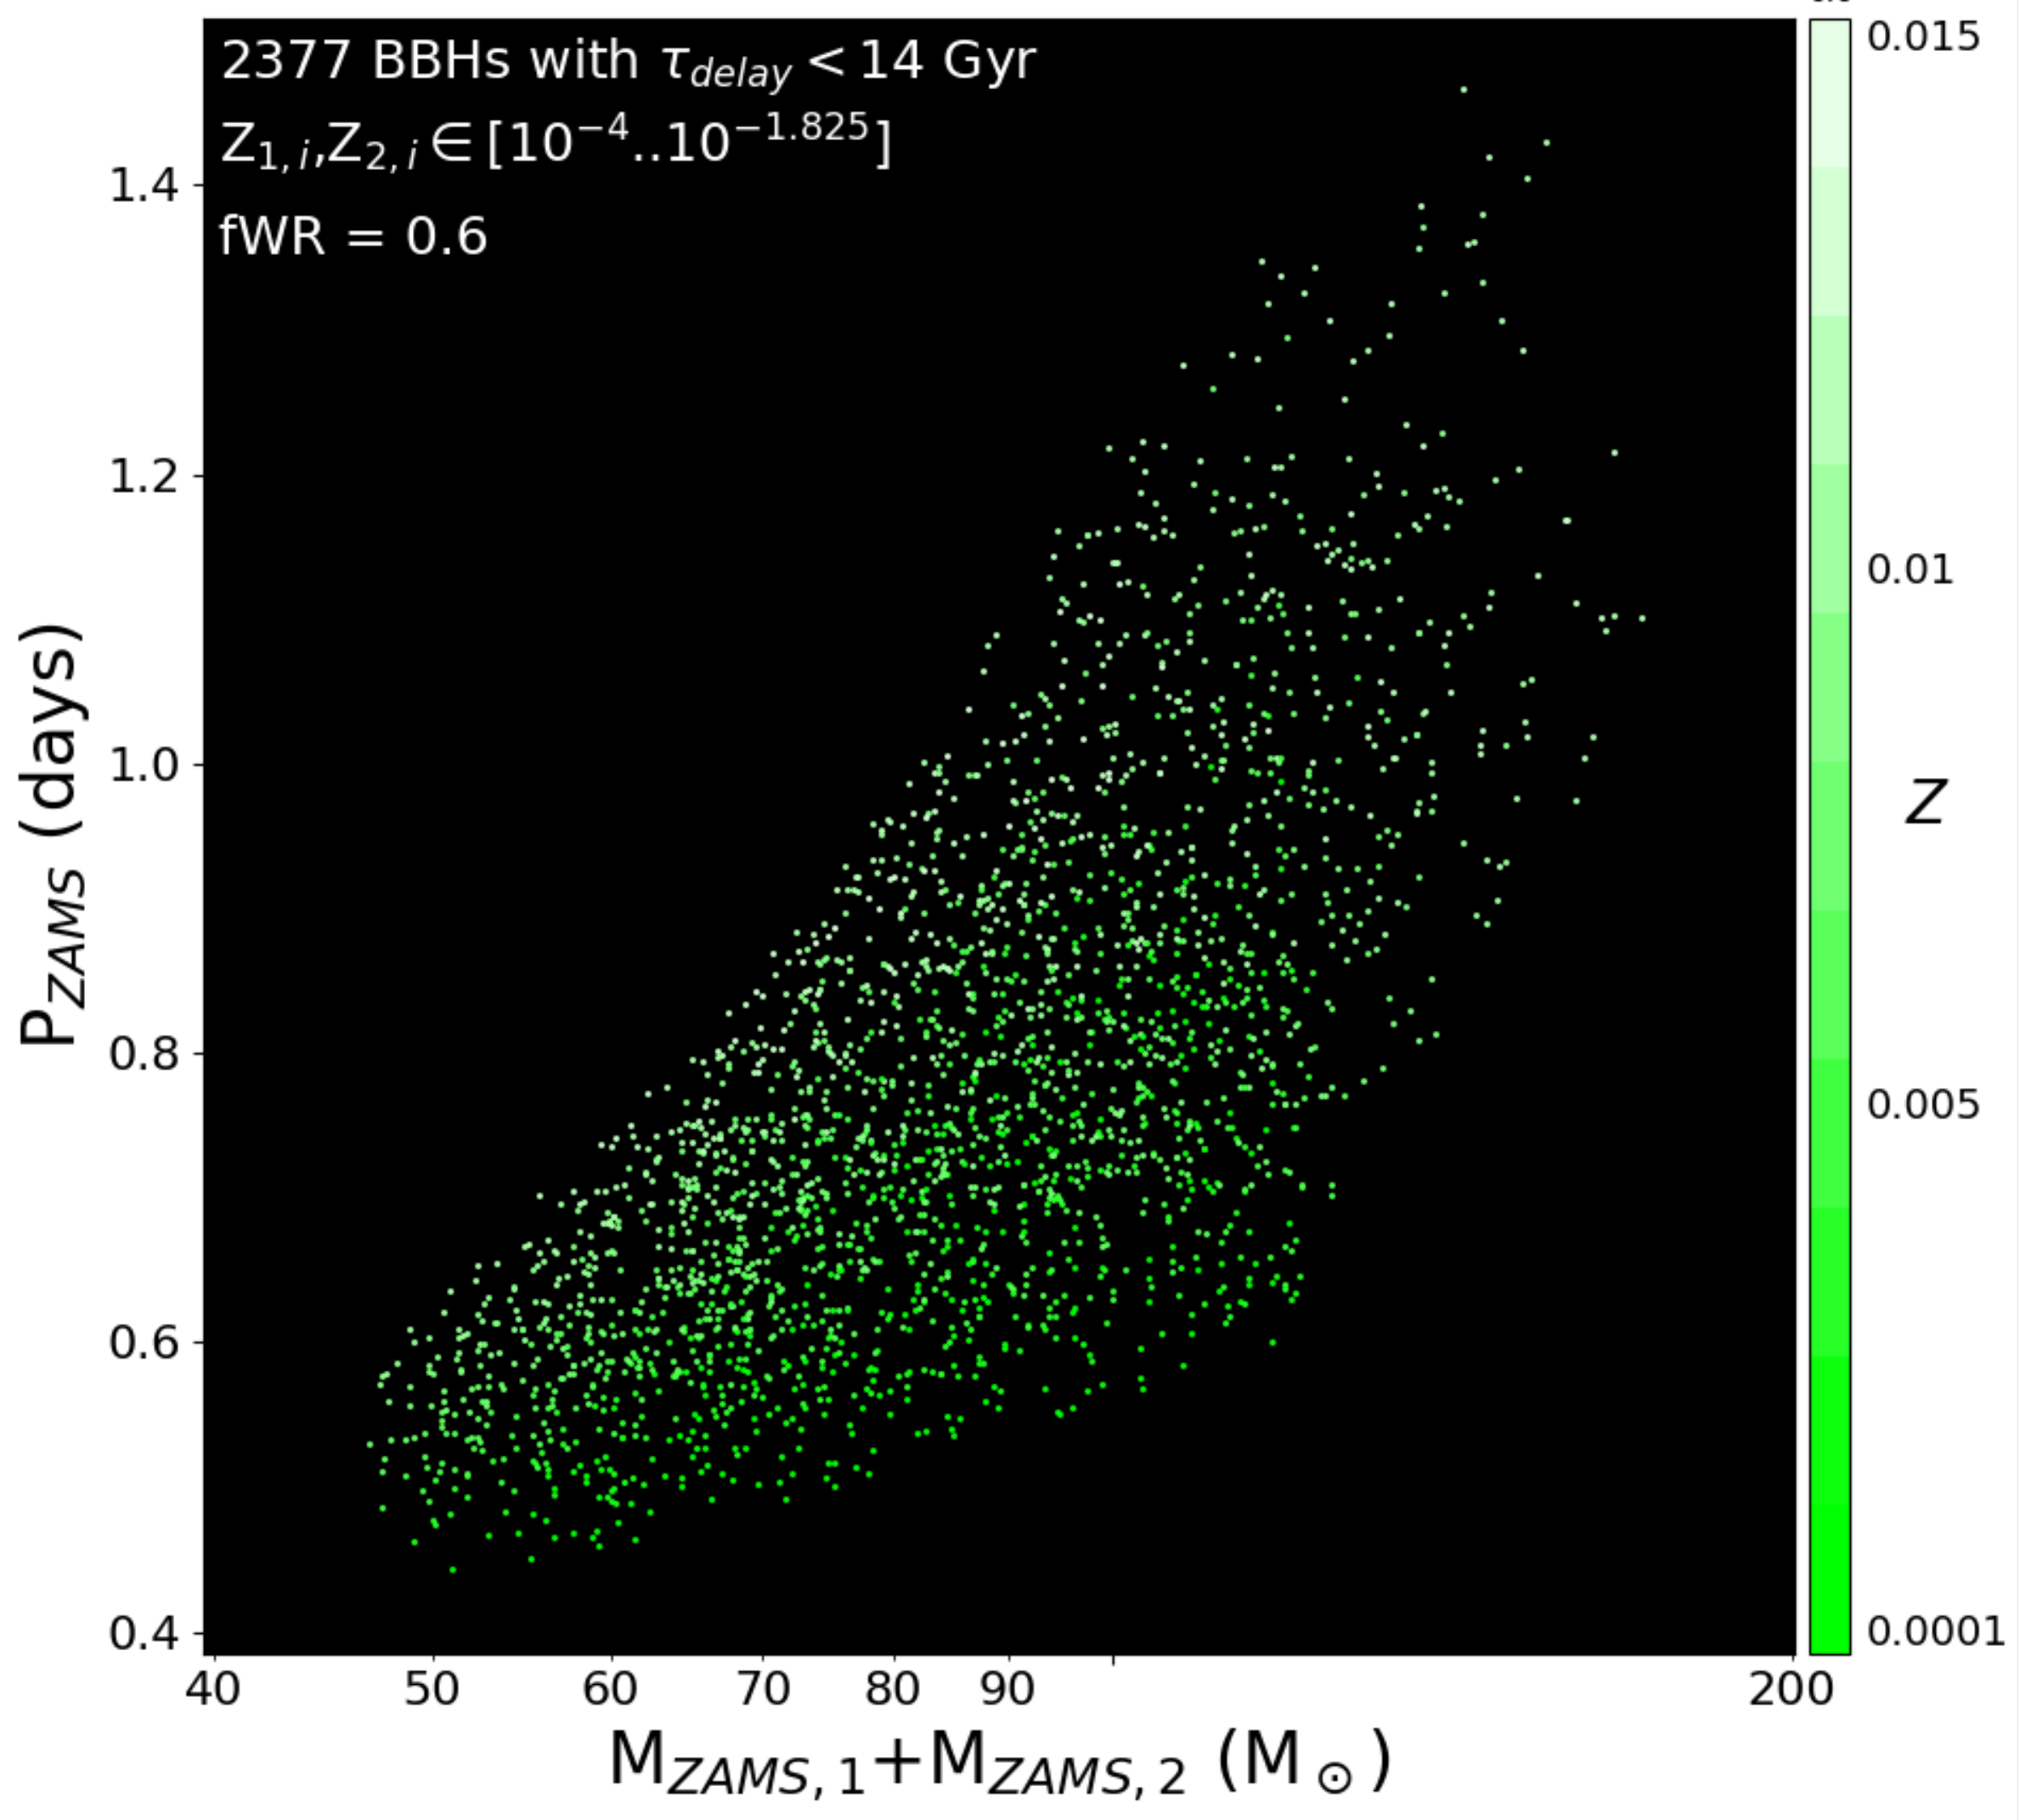}
\captionof{figure}{$f_{wr}=0.6$}
\label{fig:pInitialVSmTotal_fWR0_6}

\includegraphics[width=0.475\textwidth]{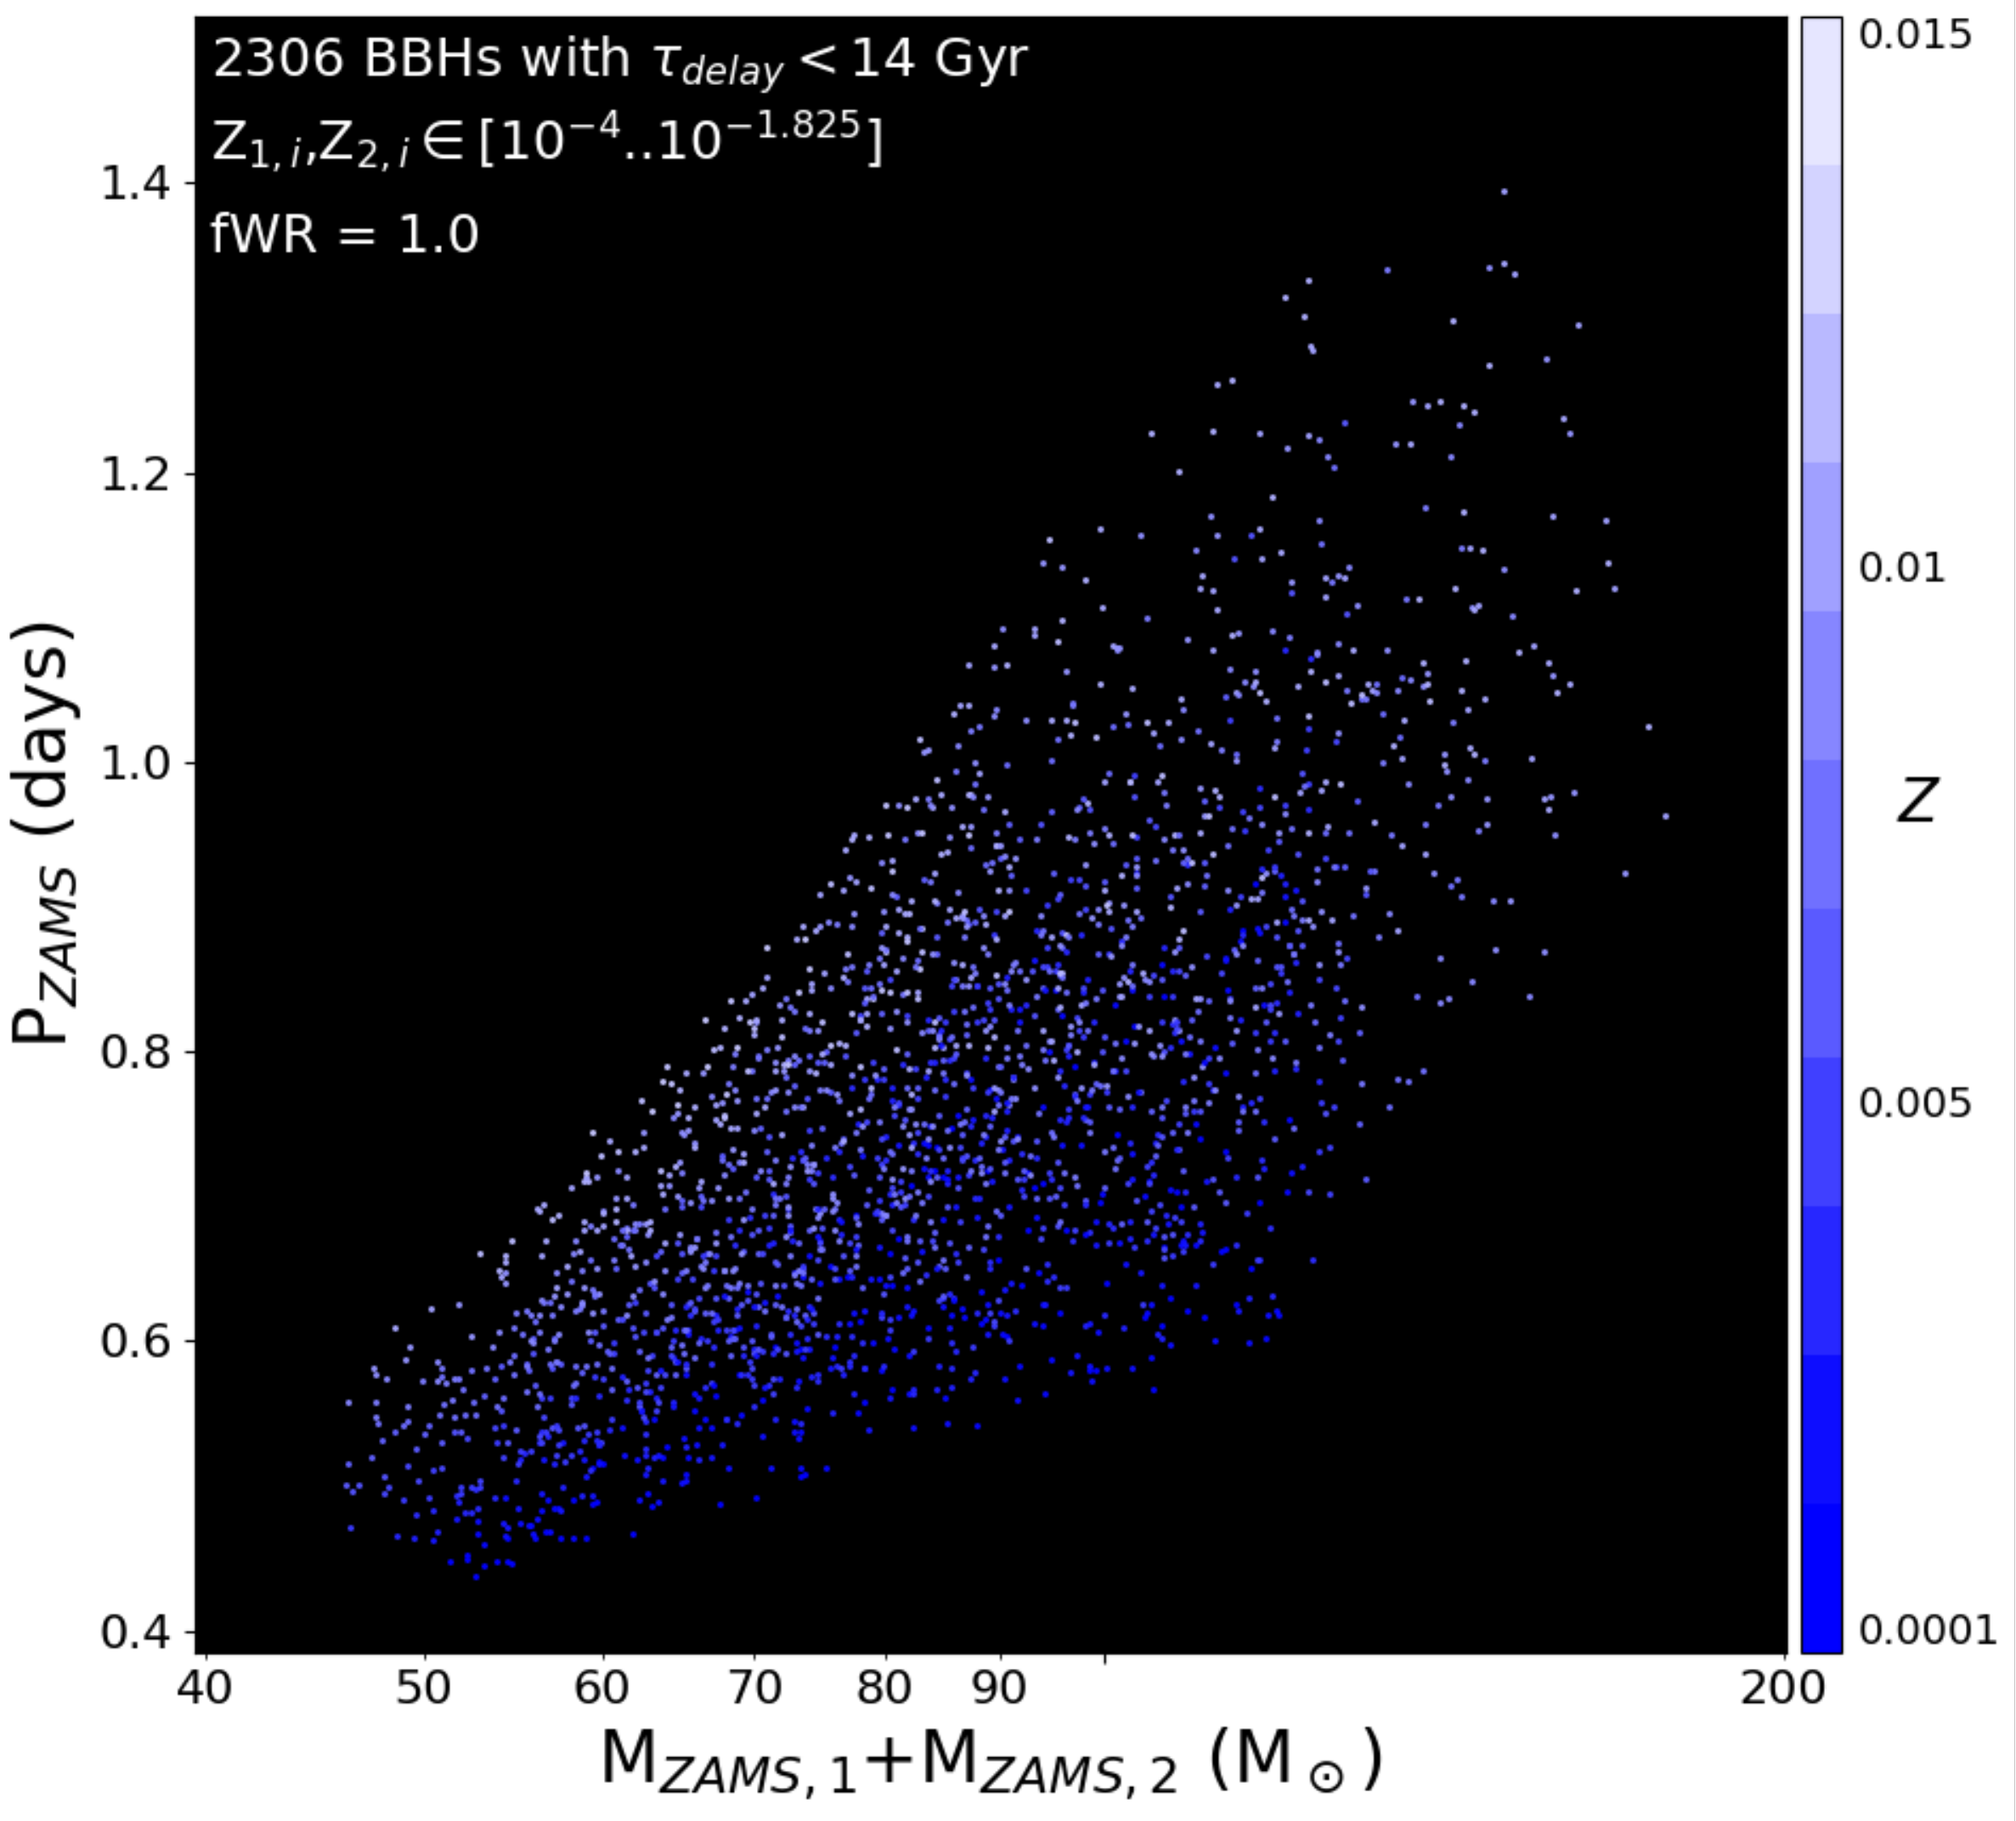}
\captionof{figure}{$f_{wr}=1.0$}
\label{fig:pInitialVSmTotal_fWR1_0}

\end{multicols}

\clearpage
\begin{multicols}{2}
\subsection{Final attributes}\label{subsec:pFinalVSmTotal_plots}

Figures~\ref{fig:pFinalVSmTotal_fWR0_0}, \ref{fig:pFinalVSmTotal_fWR0_2}, \ref{fig:pFinalVSmTotal_fWR0_6}, and ~\ref{fig:pFinalVSmTotal_fWR1_0} show final system total masses and orbital periods for \ac{CHE} systems that have formed \acp{BBH} that will merge within 14 Gyr for \ac{WR} wind factors $0.0,\ 0.2,\ 0.6,$ and $1.0$ respectively. These are the constituent plots that, when overlaid, make up Figure~\ref{fig:pFinalVSmTotal_fWRall}.

See Section~\ref{subsec:pop_synth} for a detailed description of these plots.

\end{multicols}

% forcing placement of the plots by not wrapping it in /begin{figure}.../end{figure}
\begin{multicols}{2}

\includegraphics[width=0.475\textwidth]{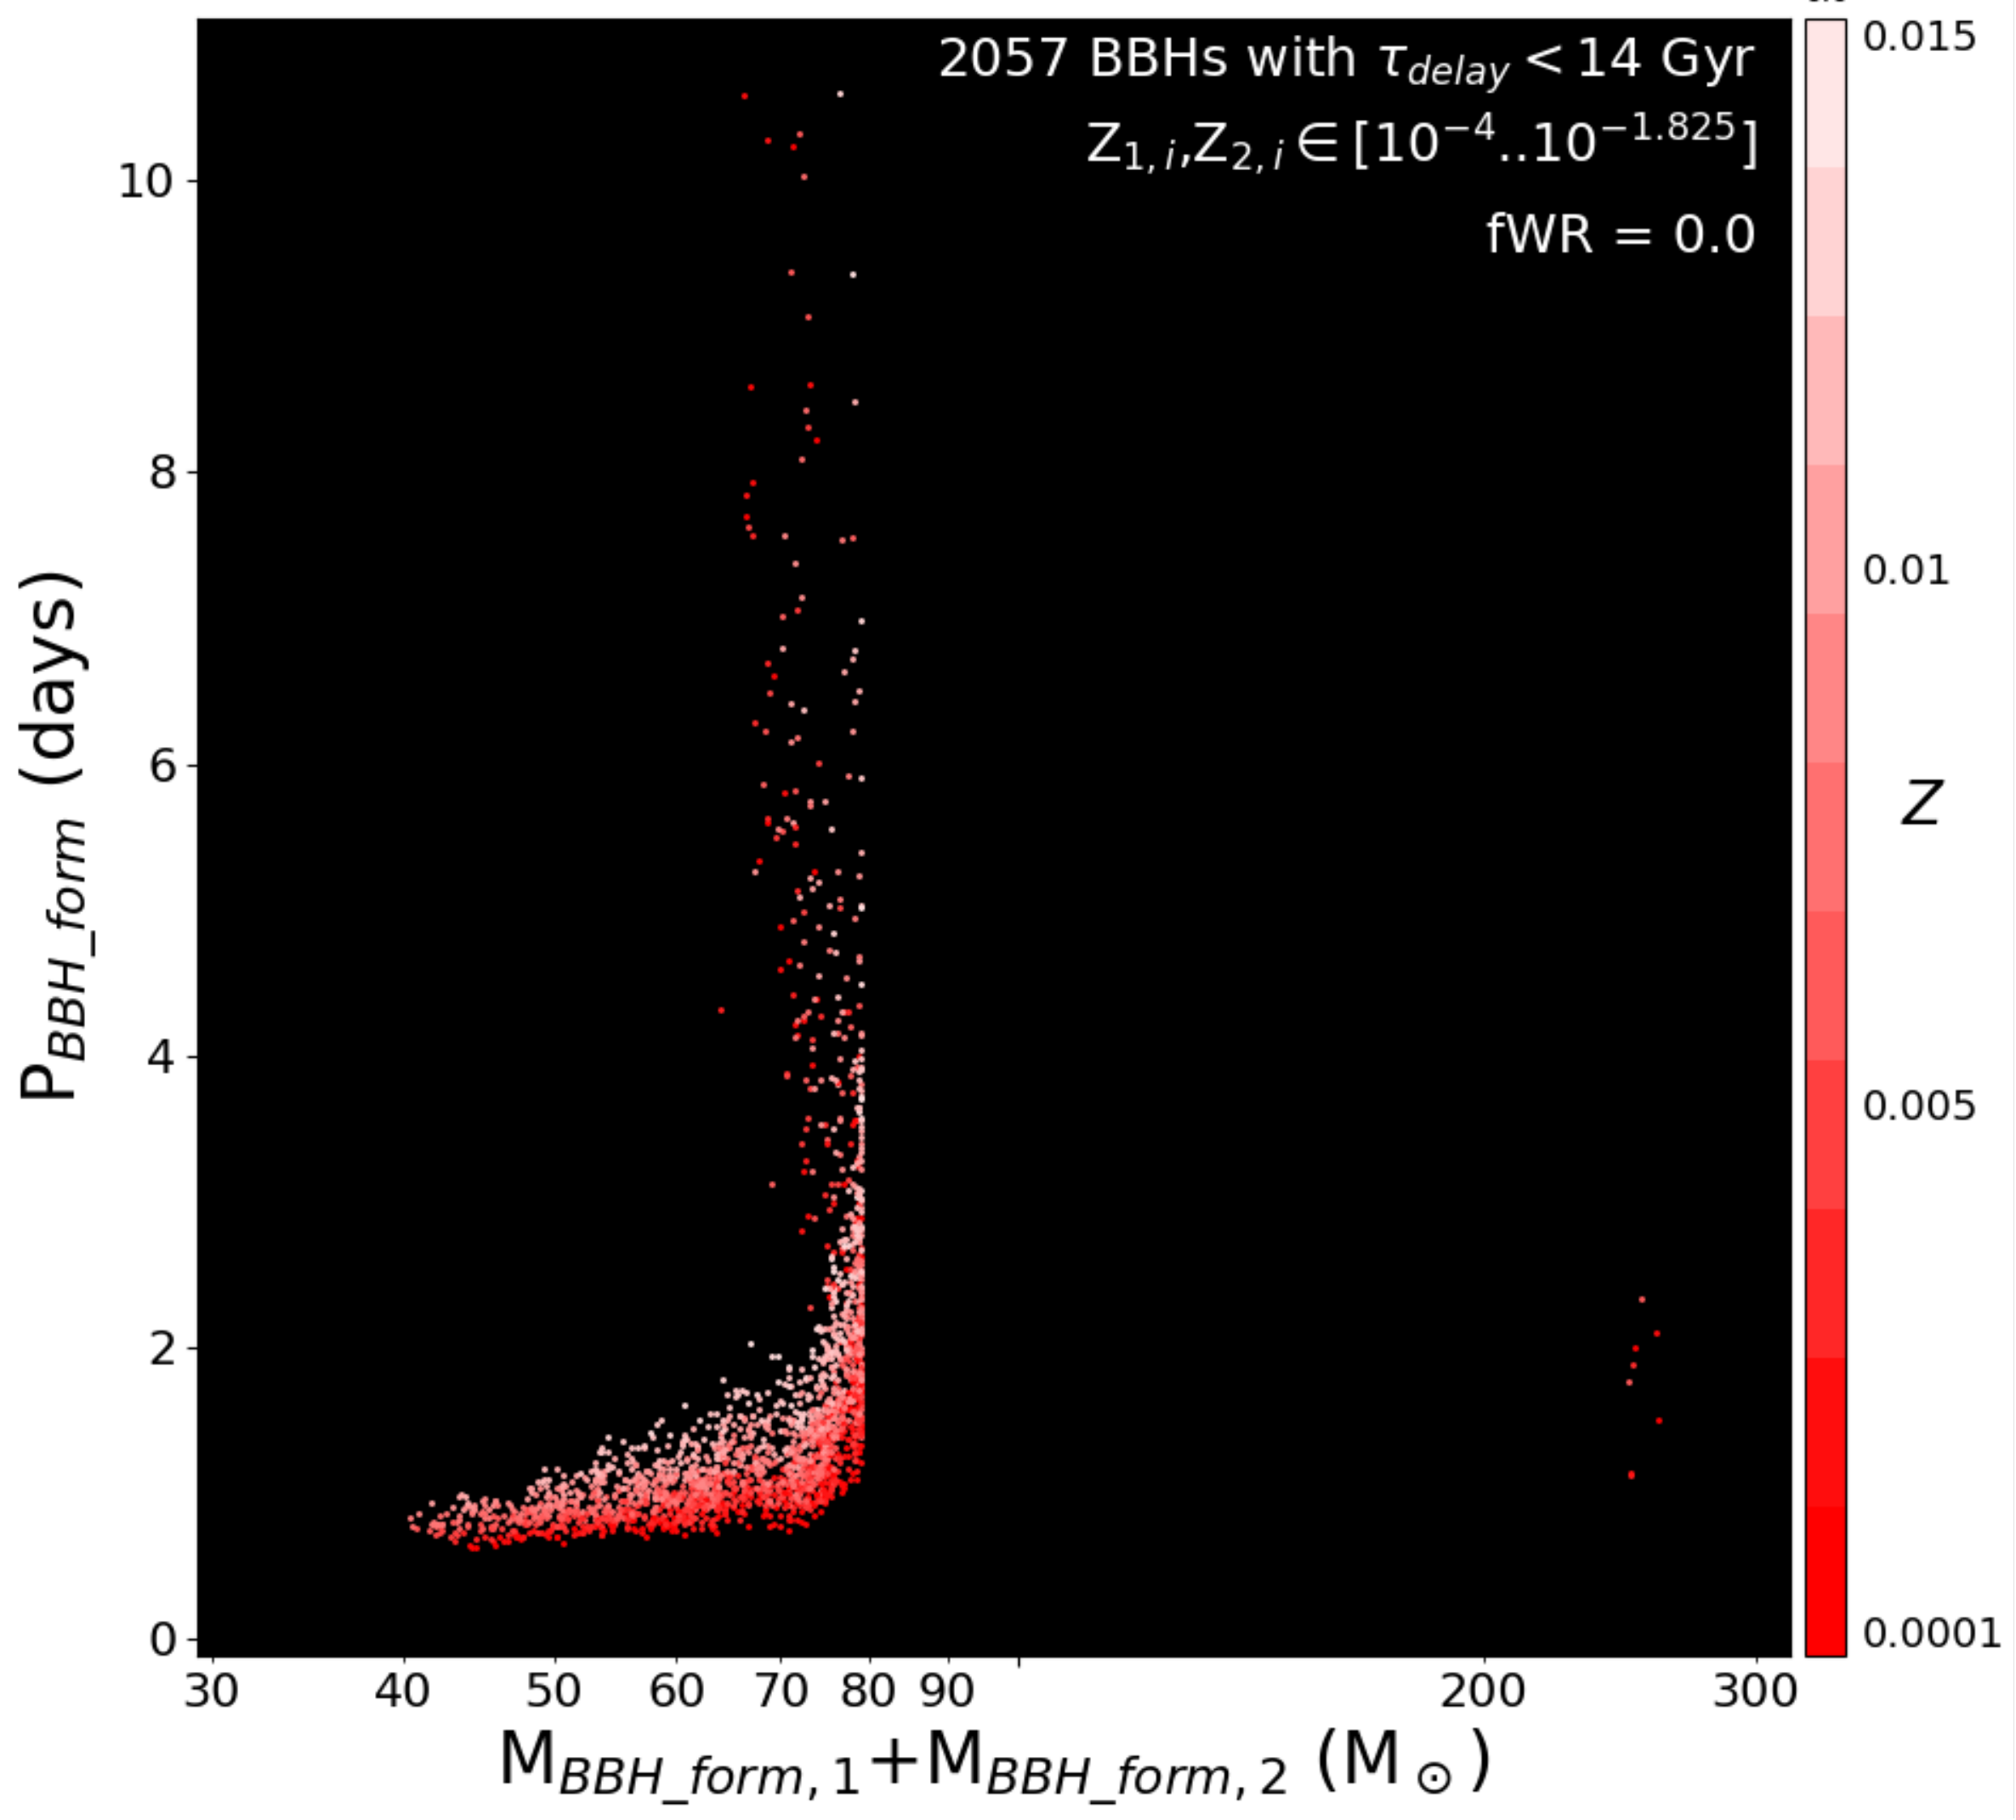}
\captionof{figure}{$f_{wr}=0.0$}
\label{fig:pFinalVSmTotal_fWR0_0}

\includegraphics[width=0.475\textwidth]{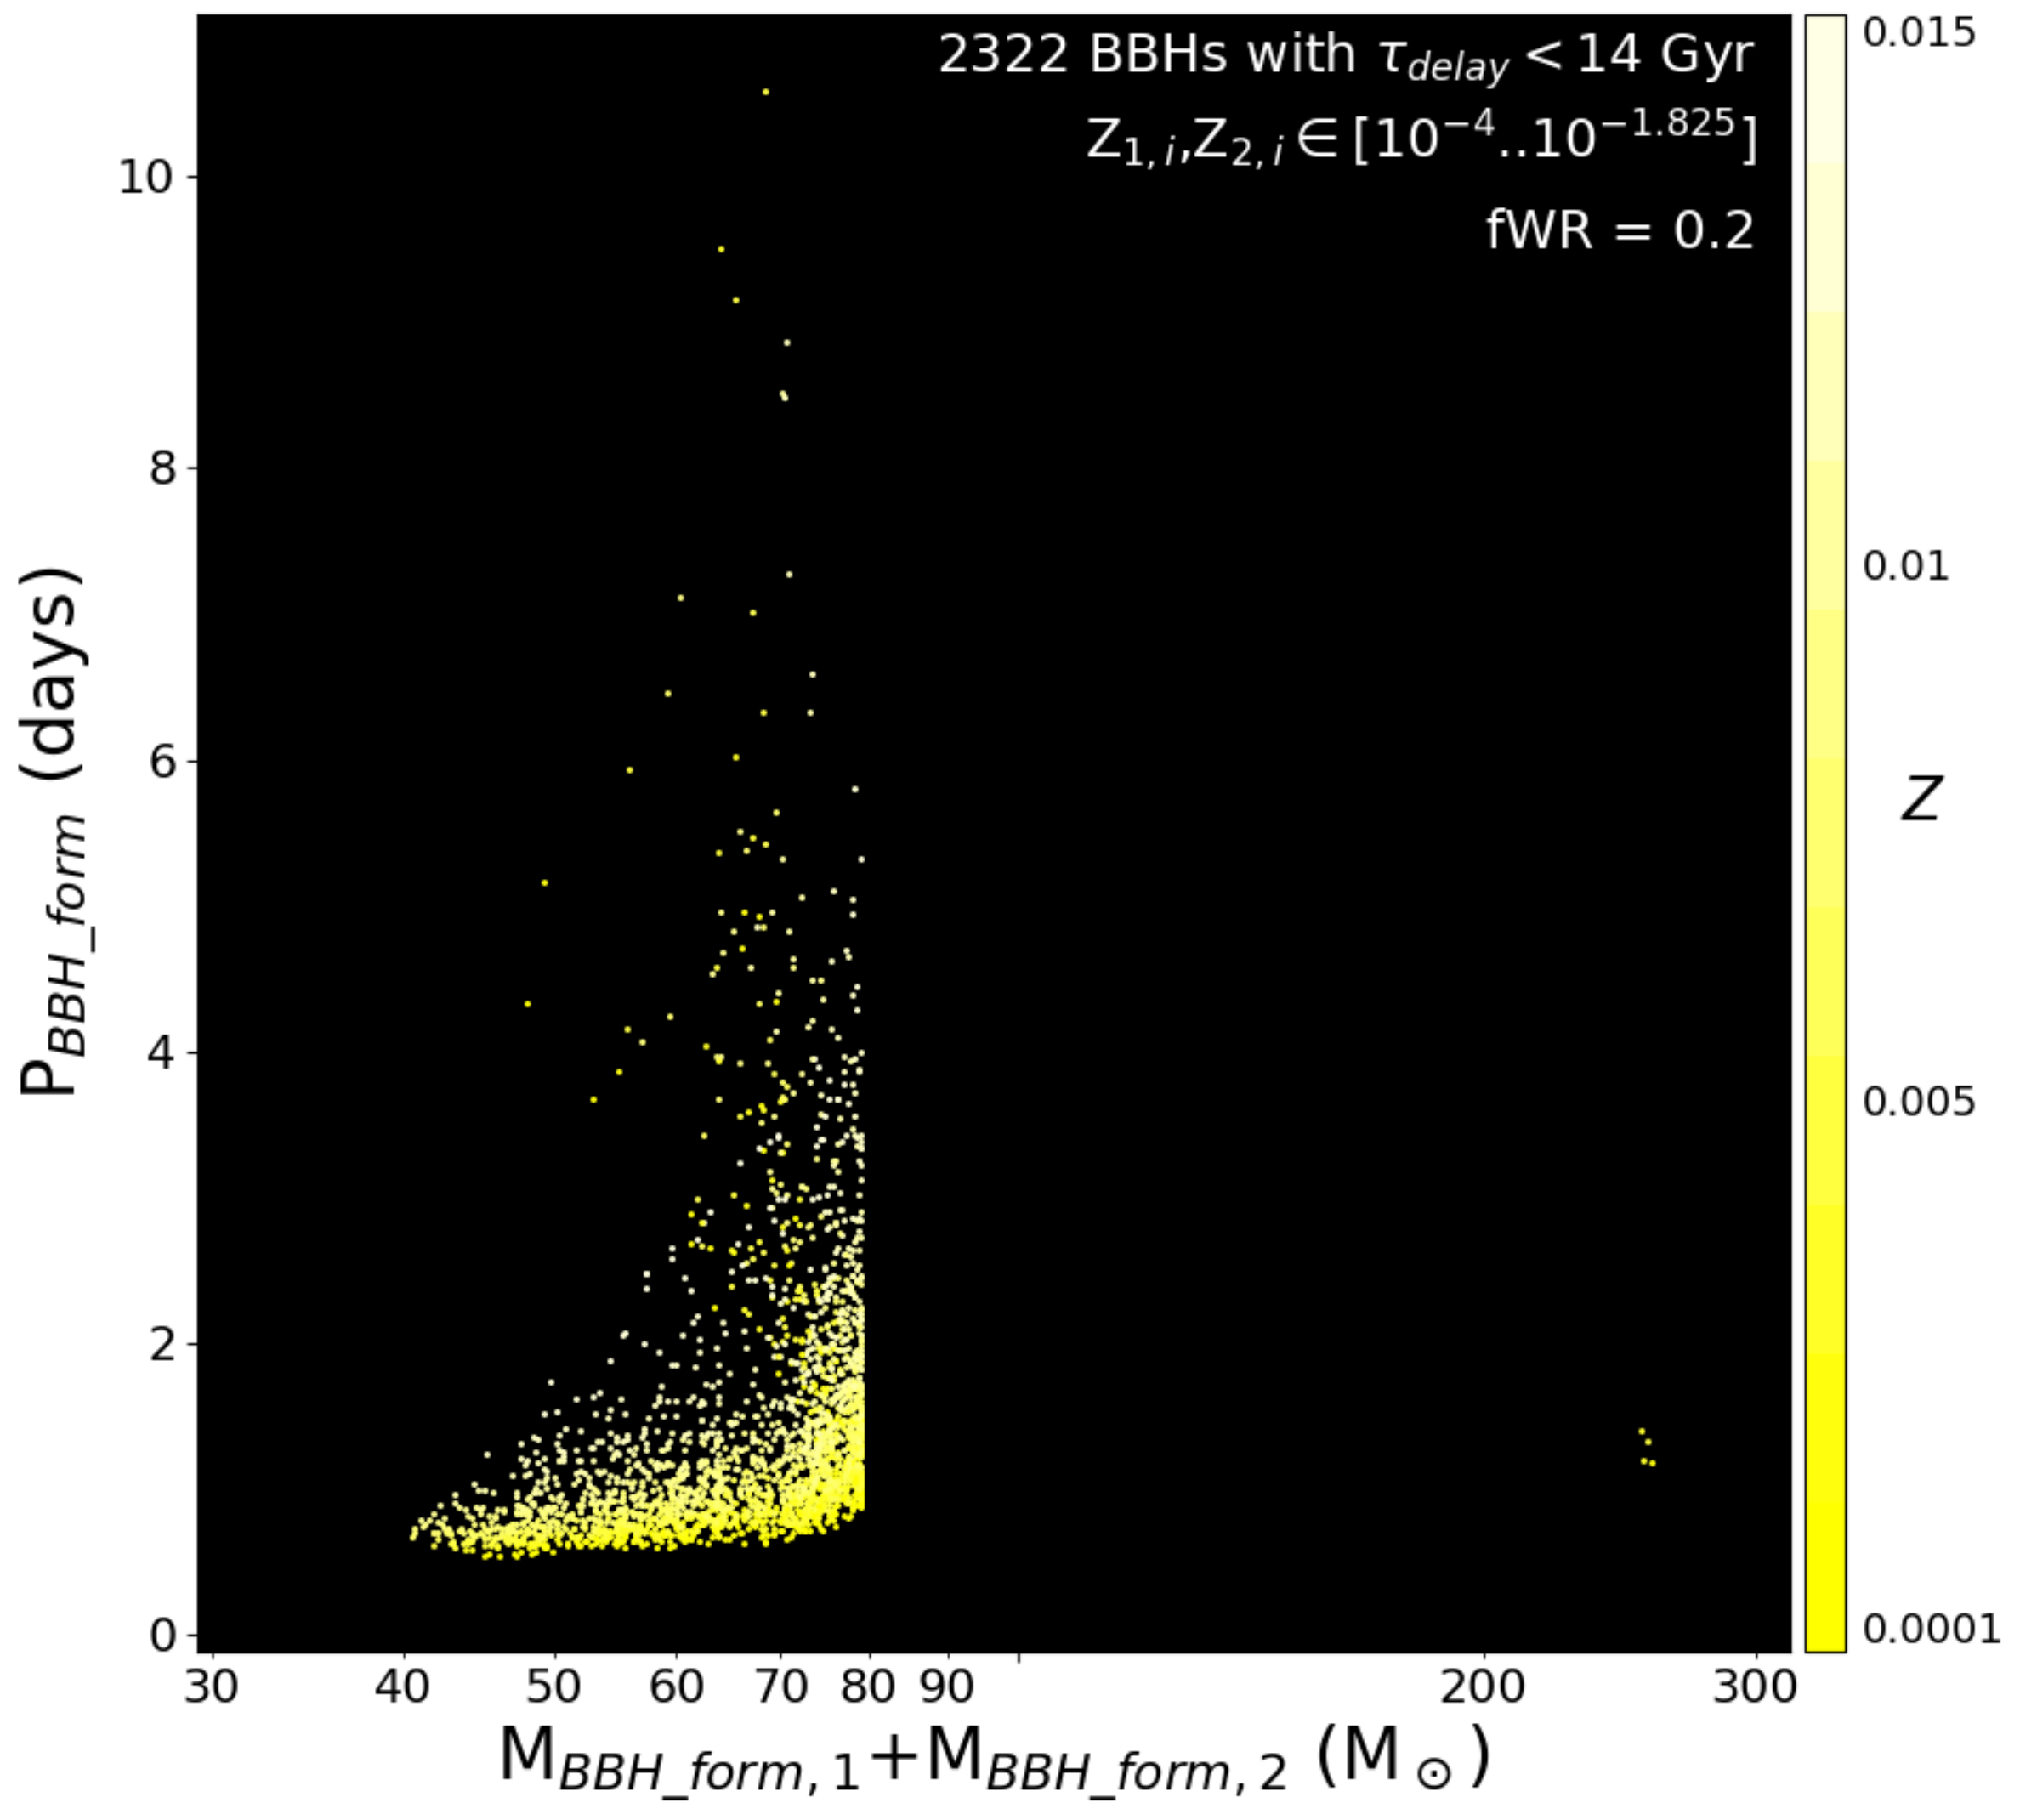}
\captionof{figure}{$f_{wr}=0.2$}
\label{fig:pFinalVSmTotal_fWR0_2}

\end{multicols}
\begin{multicols}{2}

\includegraphics[width=0.475\textwidth]{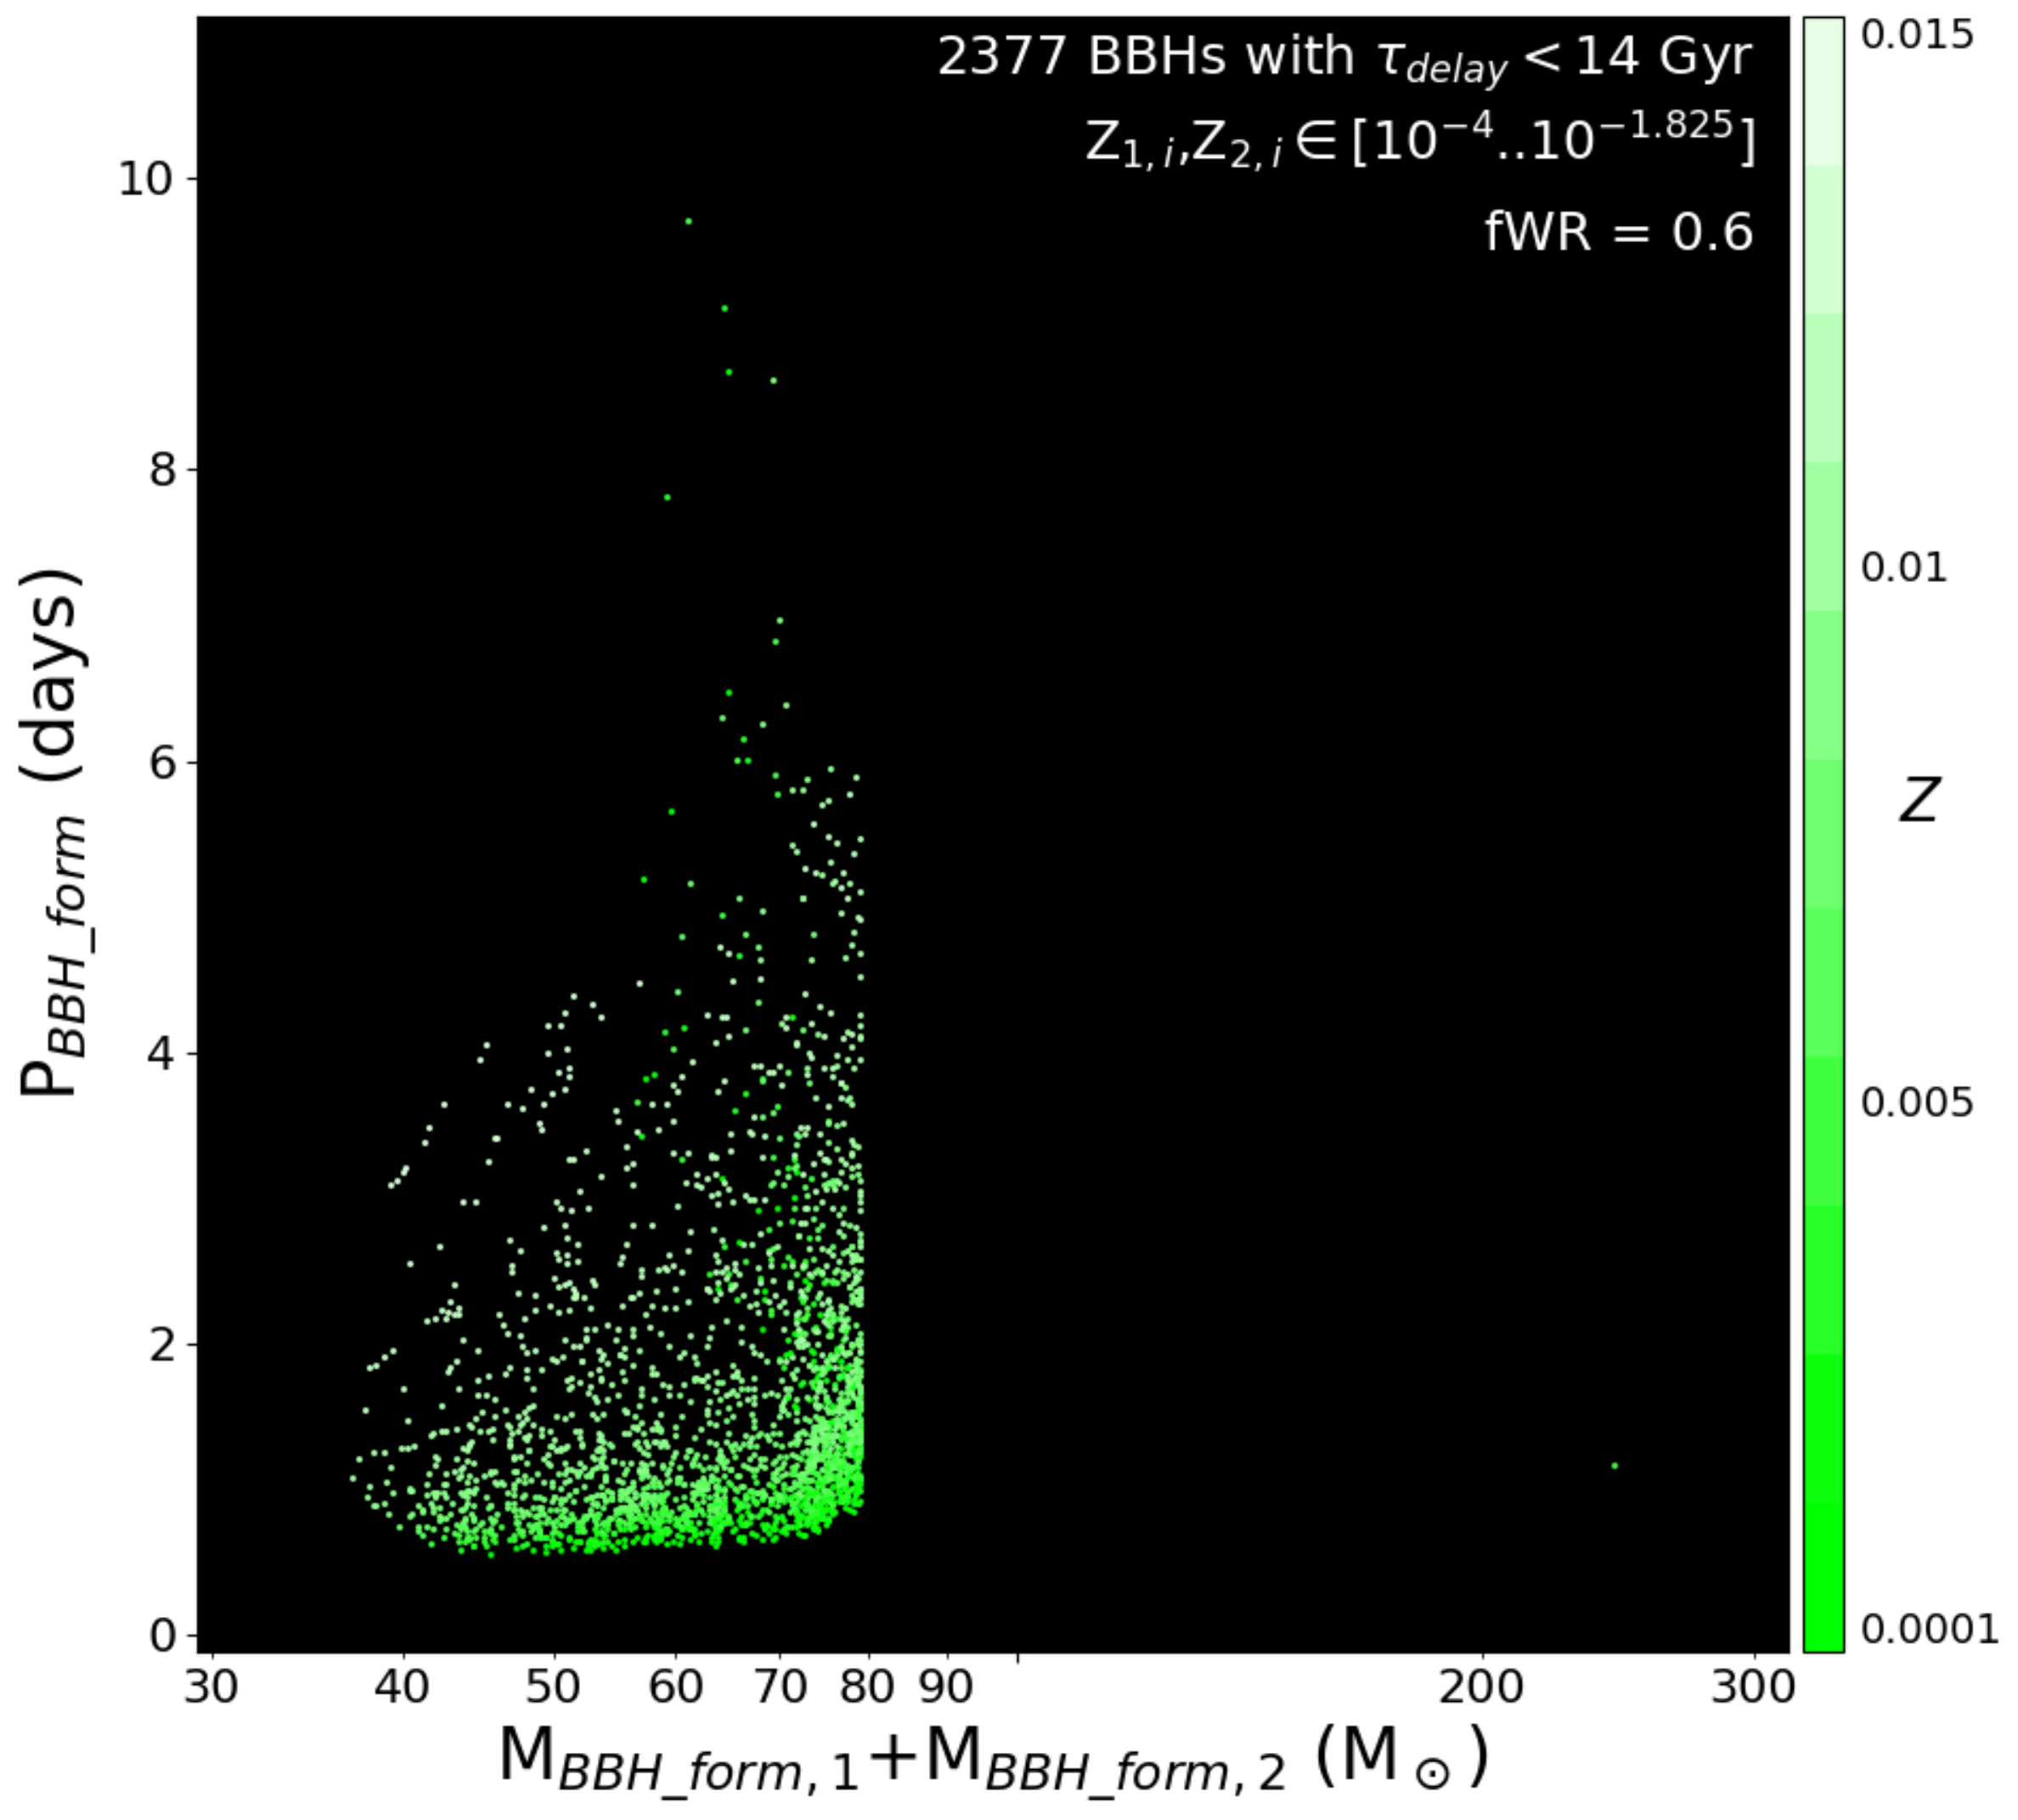}
\captionof{figure}{$f_{wr}=0.6$}
\label{fig:pFinalVSmTotal_fWR0_6}

\includegraphics[width=0.475\textwidth]{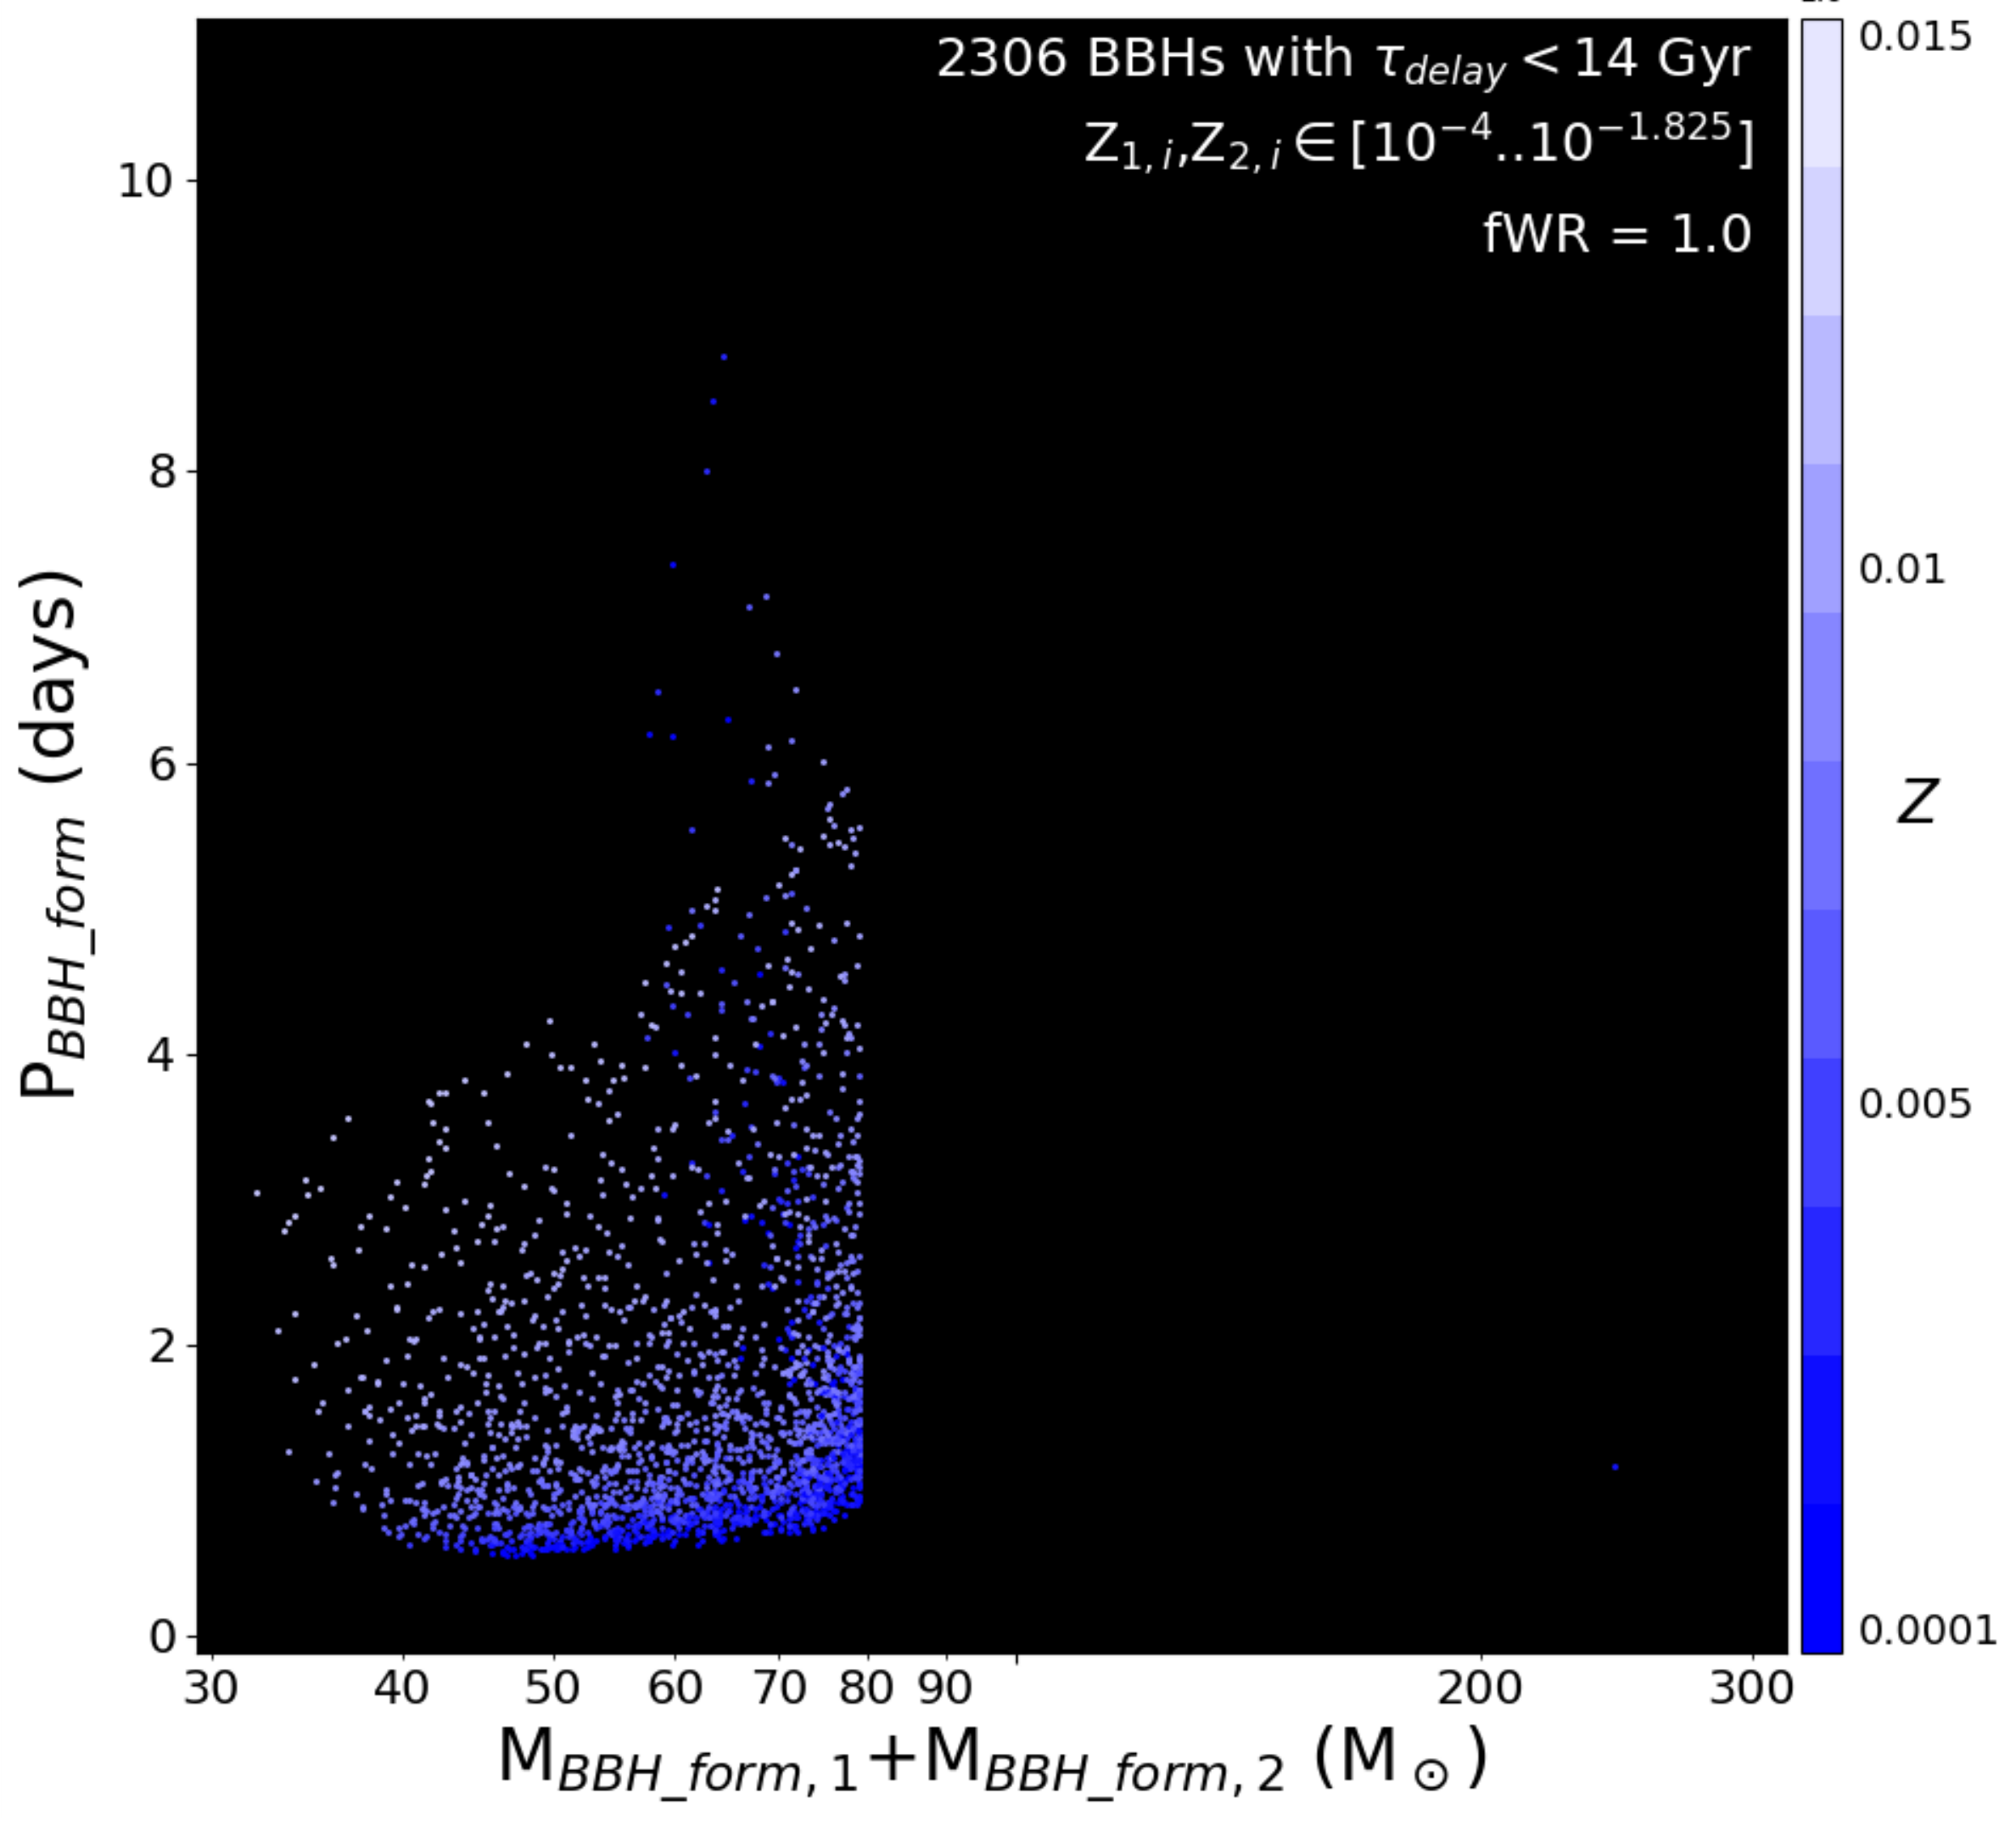}
\captionof{figure}{$f_{wr}=1.0$}
\label{fig:pFinalVSmTotal_fWR1_0}

\end{multicols}
\twocolumn
