# Supplementary material for: Chemically Homogeneous Evolution: A rapid population synthesis approach
Source: arXiv:2010.00002 source file (2021-05-02)
Supplement: Supplementary file 3 [file appendix-WRwinds.tex]

\onecolumn
\begin{multicols}{2}
\section{Wolf-Rayet wind factors}\label{sec:WolfRayetWinds}

Figure~\ref{fig:BBH_yield} (Section~\ref{subsubsec:results_formation_rates}) shows the \ac{BBH} formation rate per unit star forming mass as a function of metallicity for systems that form \acp{BBH} that will merge within the age of the universe, and seems to indicate that \ac{WR} wind strength has minimal impact on the formation rate, for both the full population (both \ac{CHE} and non-\ac{CHE} binaries; solid lines) and the \ac{CHE} binaries only (dashed lines).

Figure~\ref{fig:WRMassLossRate} shows the mass loss rate due to \ac{WR} winds, as calculated using Equation~\ref{eqn:WRwinds}, for a \ac{WR} star with \mbox{$L=1.3\tenpow{6}L_{\odot}$} (with indicative mass $\sim40\Msun$). We show mass loss rates for \mbox{$f_{wr}\in\{\,0.0, 0.2, 0.6, 1.0, 5.0, 10.0\,\}$}. We surmise from Figures~\ref{fig:BBH_yield}~and~\ref{fig:WRMassLossRate} that the mass loss rate induced by \ac{WR} winds is not sufficient to reduce the mass of the constituent stars of binary systems, or widen binaries, enough to affect the formation rate of \acp{BBH} appreciably when $f_{wr}\leq1.0$.

To test the effect of stronger \ac{WR} winds we synthesised a further 6 million binary systems: 3 million with $f_{wr}=5.0$, and 3 million with $f_{wr}=10.0$, with thirty different metallicities evenly spaced across the range \mbox{$\minus4\leq\logten{Z}\leq\minus1.825$}. Figure~\ref{fig:formationYield_ALL} shows the \ac{BBH} formation rate per unit star forming mass as a function of metallicity for \mbox{$f_{wr}\in\{\,0.0, 0.2, 0.6, 1.0, 5.0, 10.0\,\}$}.  

We see from Figure~\ref{fig:formationYield_ALL} that very strong \ac{WR} winds do affect the formation rate of \acp{BBH} significantly. When viewed in conjunction with Figure~\ref{fig:WRMassLossRate} it is clear that the mass loss rates induced by $f_{wr}\leq1.0$ don't vary much below 0.1\Zsun, and at \Zsun the variation is not large. The lack of variation in mass loss rate for low metallicities is consistent with Equation~\ref{eqn:WRwinds}, and explains the small effect varying $f_{wr}$ has on the \ac{BBH} formation rate.

Figure~\ref{fig:WRActualMassLoss} shows the actual mass lost for a star with \ac{ZAMS} mass $\sim~40~\Msun$ during the \acf{WR} phase, for a range of \ac{WR} winds factors and metallicities. Figure~\ref{fig:WRActualMassLoss} also shows the mass and luminosity of the star at the start of the \acf{WR} phase. We can see from Figure~\ref{fig:WRActualMassLoss} that mass loss due to \ac{WR} winds is less significant at low metallicities than it is at high metallicities, and even at \Zsun the total mass lost during the \ac{WR} phase is $\sim$half the mass of the star. At low metallicities, and so at higher redshifts, the mass lost during the \ac{WR} phase is a small faction of the total mass of the star for all \ac{WR} factors, and it is only as metallicity rises that we see the curves for the different \ac{WR} factors diverge significantly.

\end{multicols}

% forcing placement of the plots by not wrapping them in /begin{figure}.../end{figure}
\begin{multicols}{2}

\includegraphics[width=0.475\textwidth]{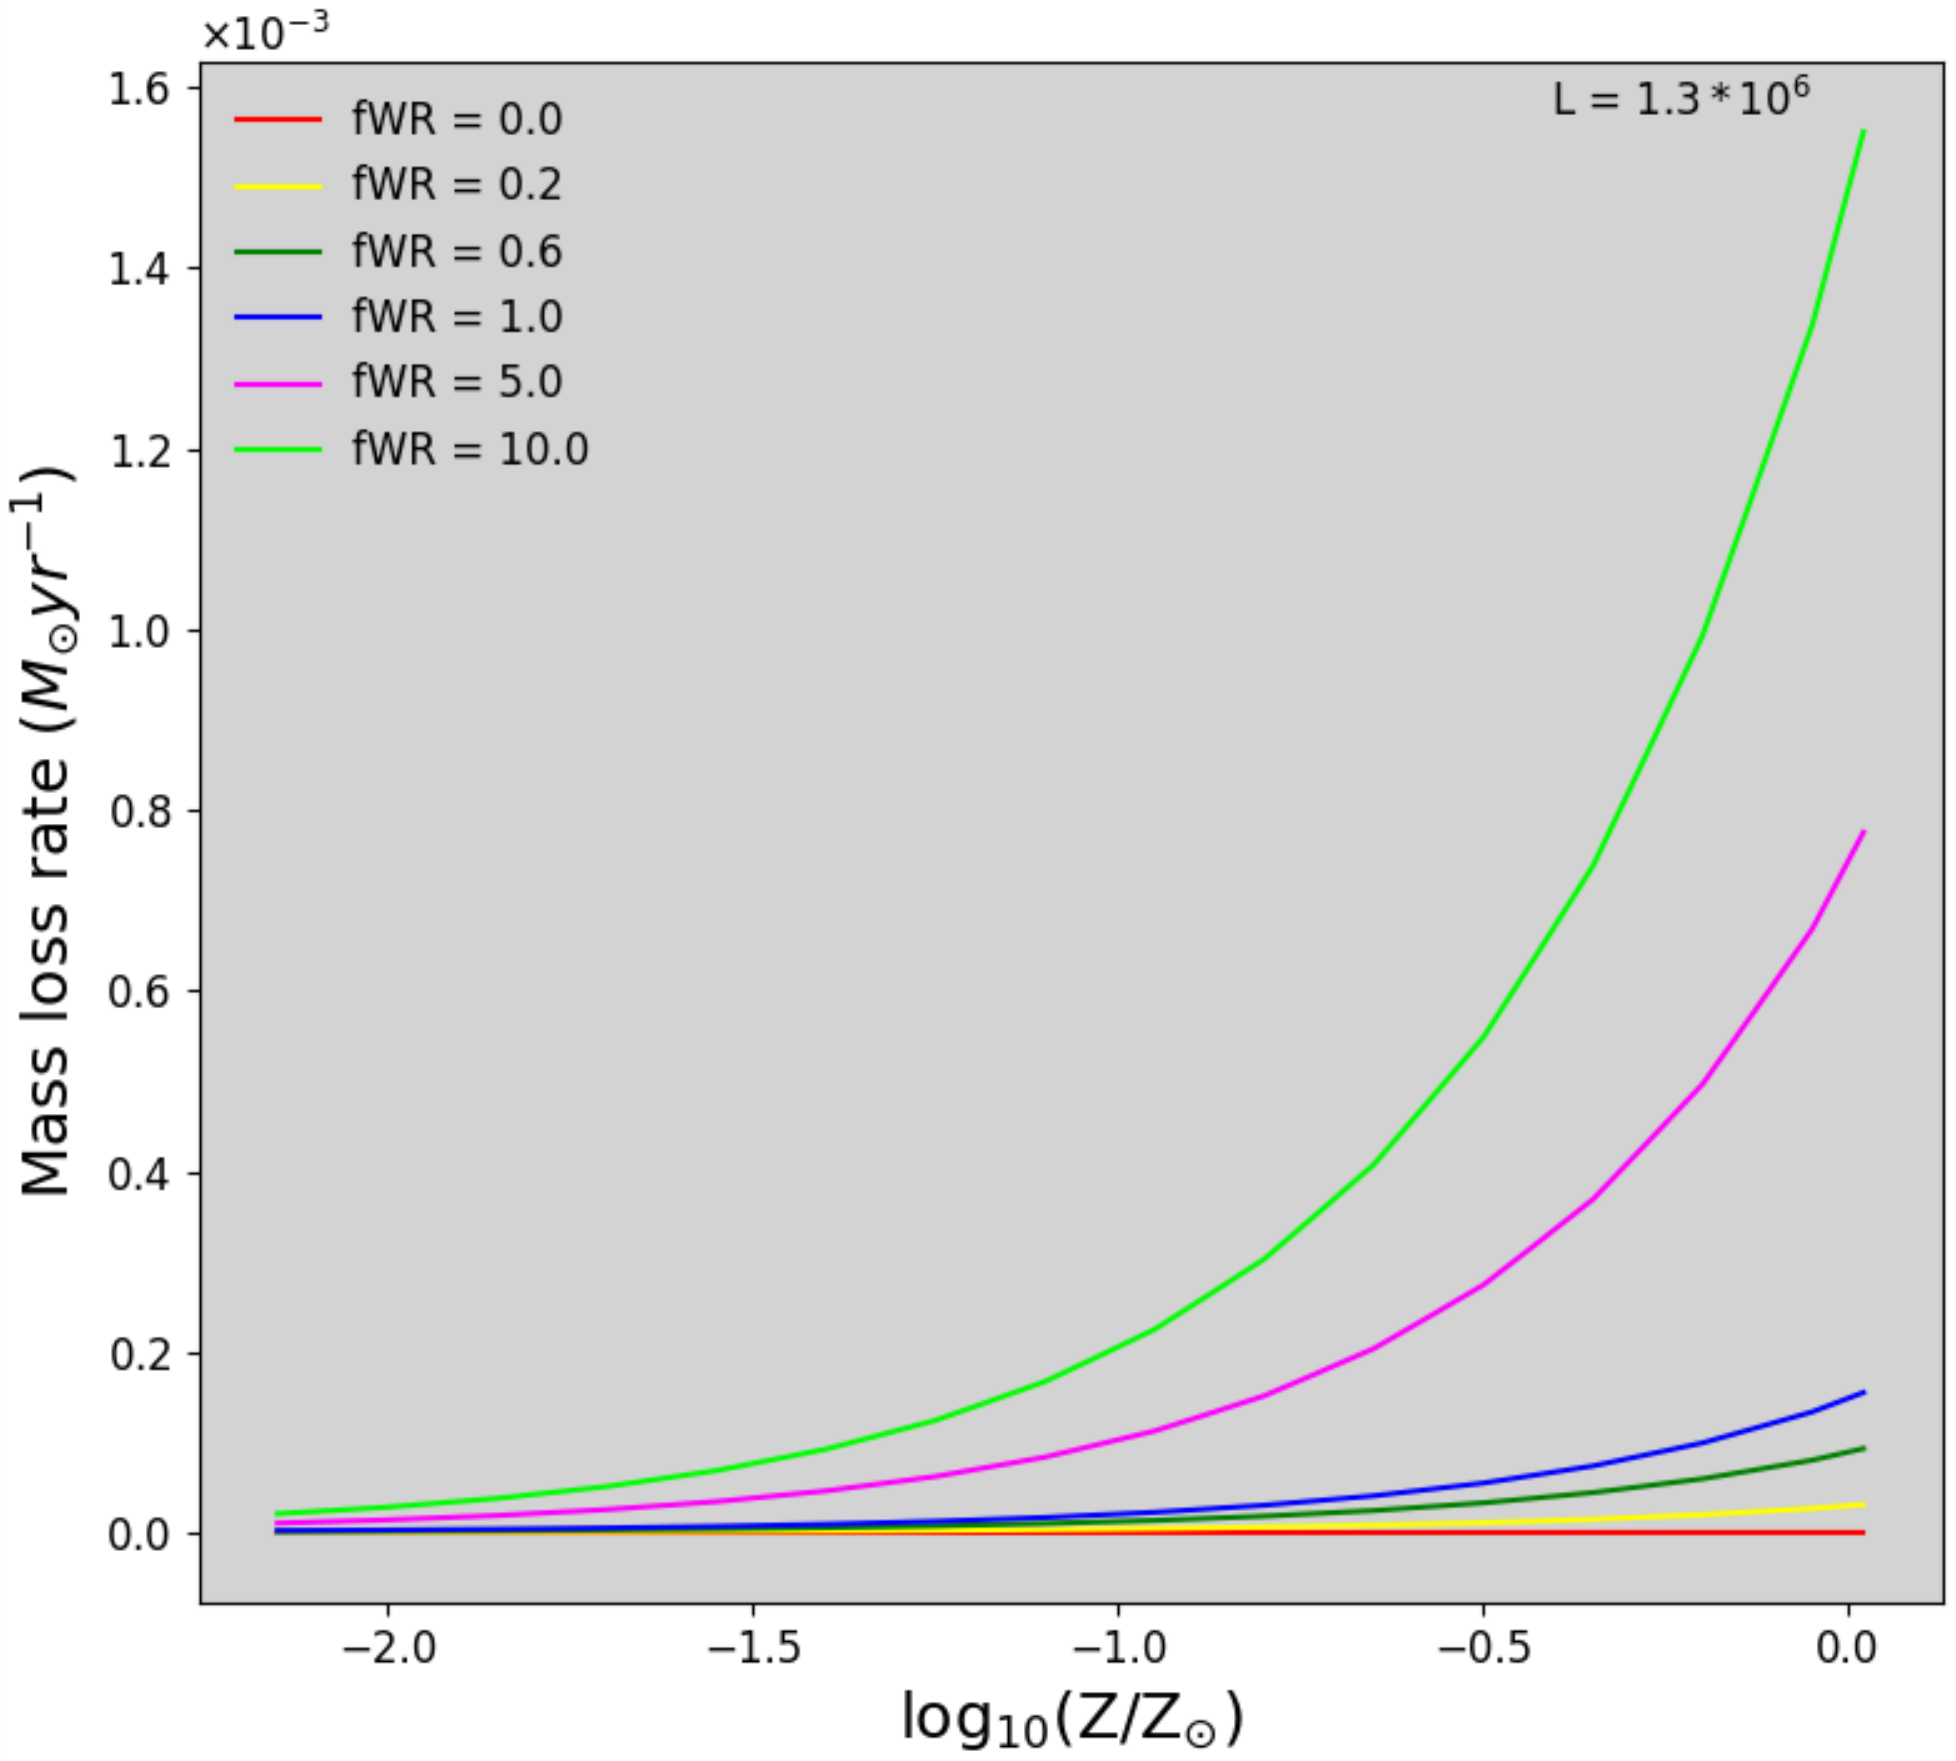}
\captionof{figure}{Mass loss rate as a function of metallicity, for a $40 \Msun$ \ac{WR} star with luminosity $L=1.3\tenpow{6}\ \mathrm{L}_\odot$. Line colour indicates the \ac{WR} mass loss rate multiplier $f_\mathrm{WR}$.}
\label{fig:WRMassLossRate}

\includegraphics[width=0.475\textwidth]{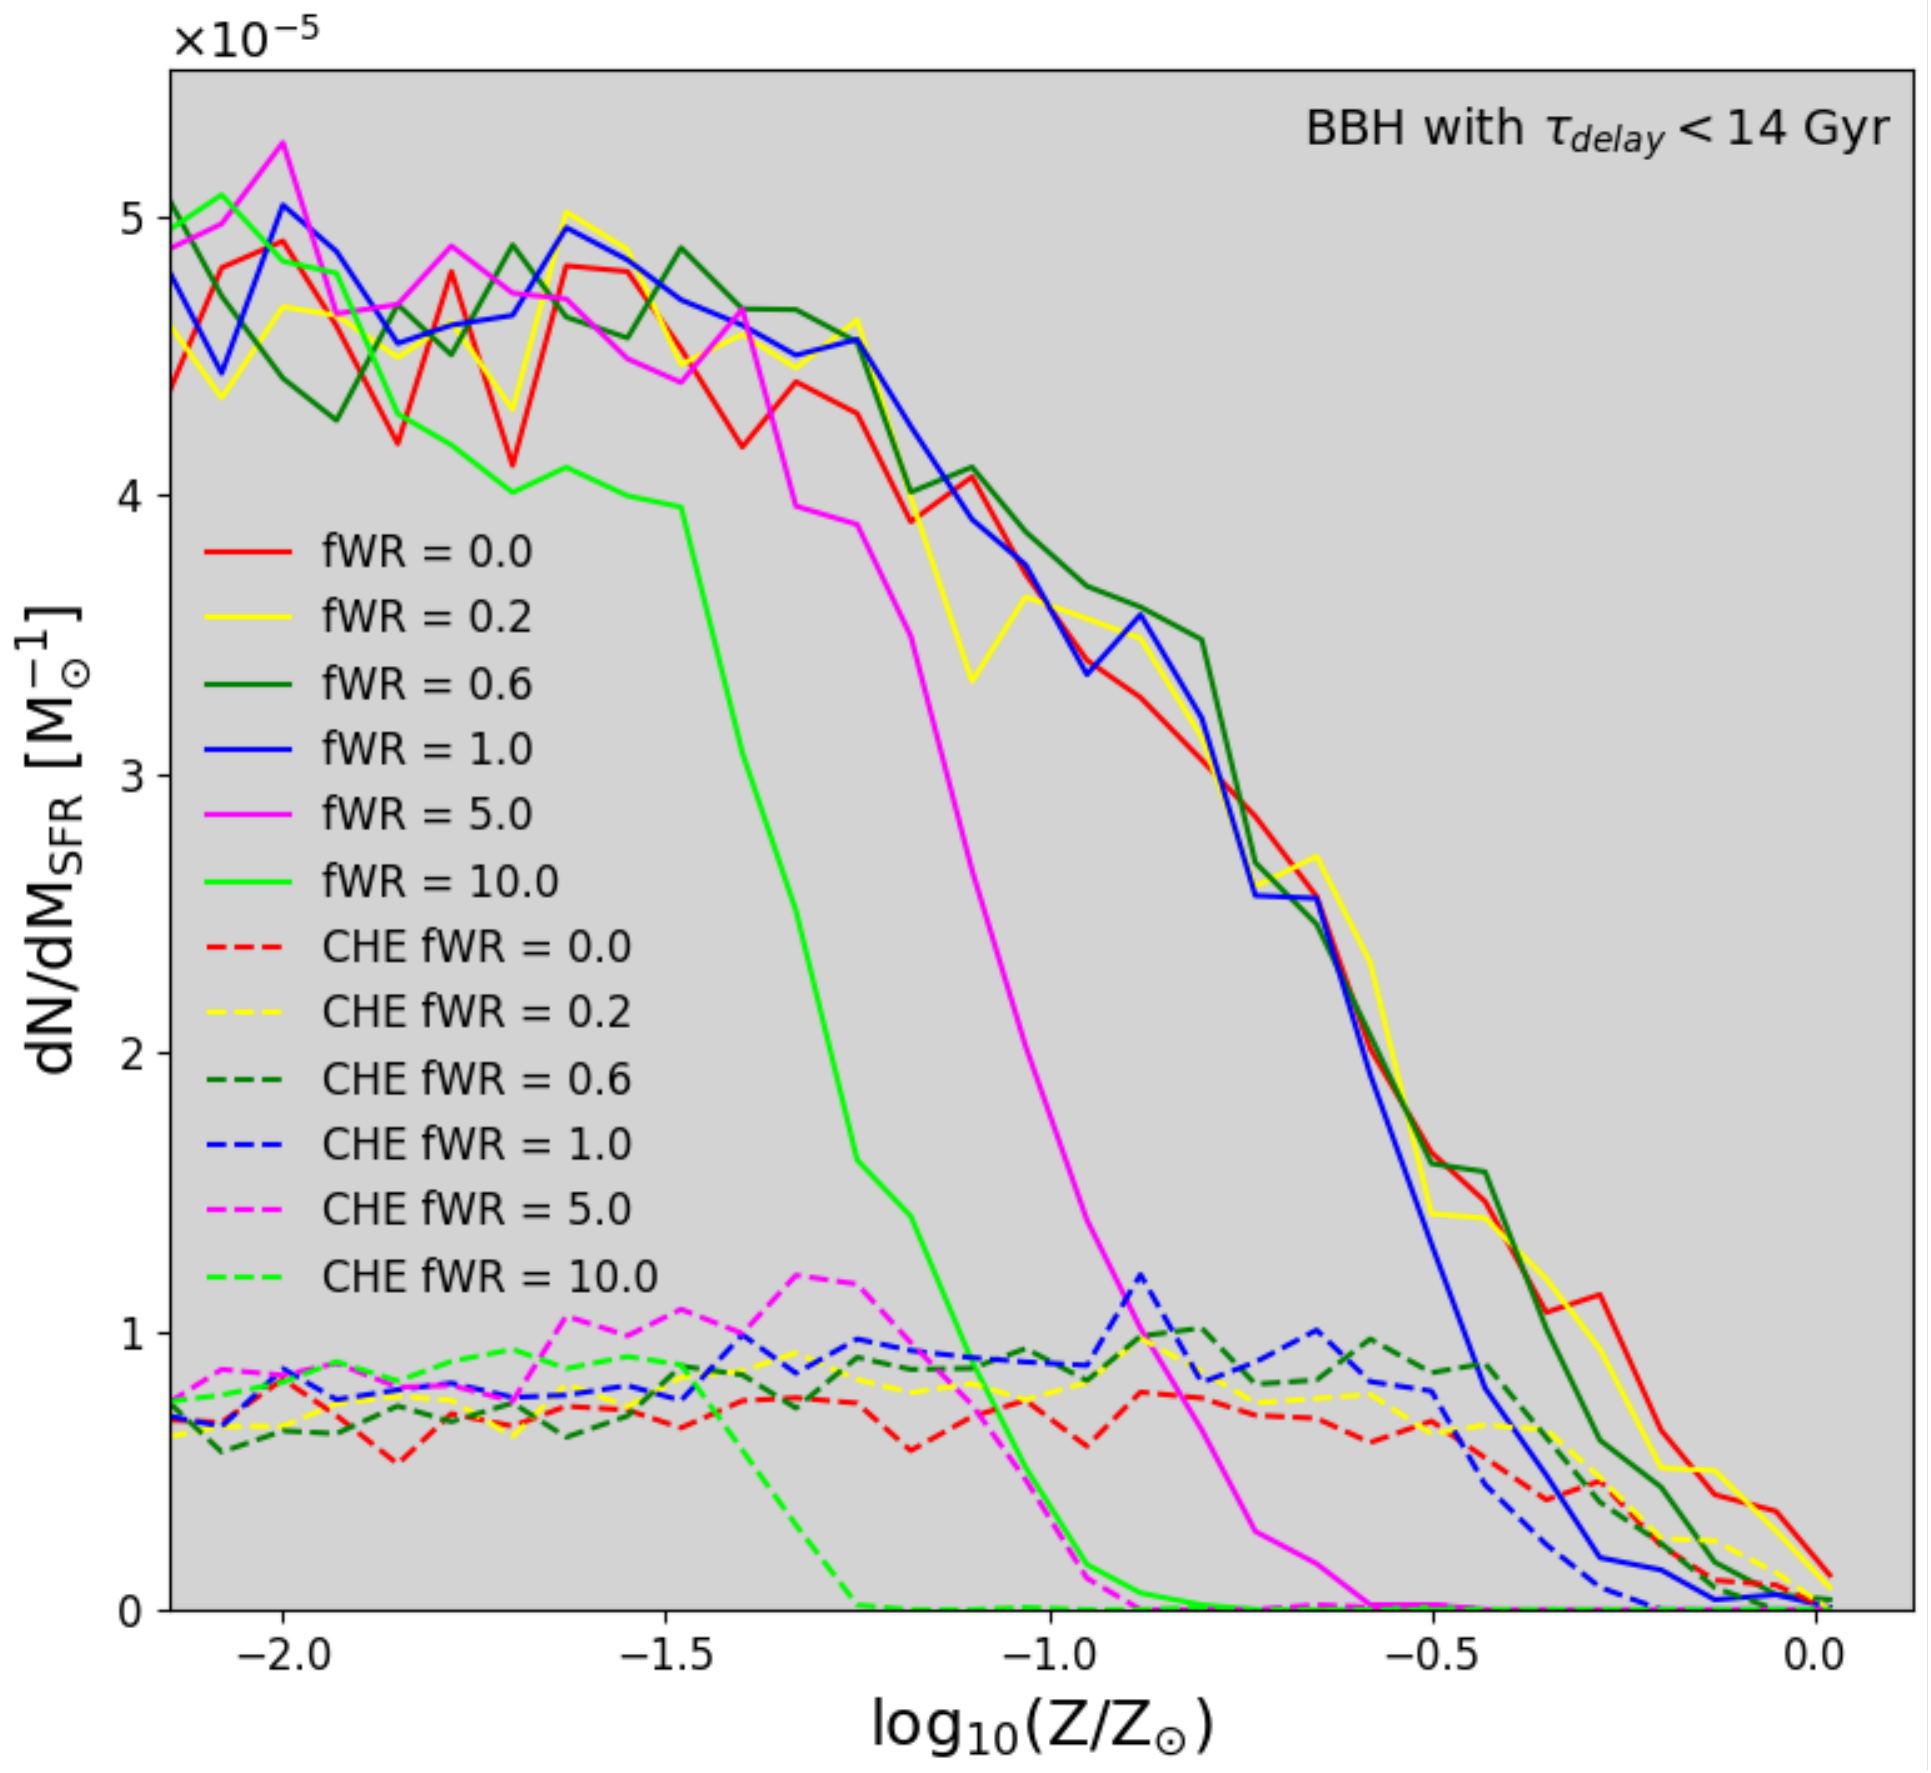}
\captionof{figure}{\ac{BBH} yield per unit star formation, as a function of metallicity. Line colour indicates the \ac{WR} mass loss rate multiplier; solid lines are all \acs{BBH}, dashed lines are \ac{CHE} \acp{BBH}. This plot is similar to Figure \ref{fig:BBH_yield} but includes $f_\mathrm{WR}=5$ and $f_\mathrm{WR}=10$ curves.}
\label{fig:formationYield_ALL}

\begin{minipage}{\linewidth}
    \includegraphics[width=\textwidth]{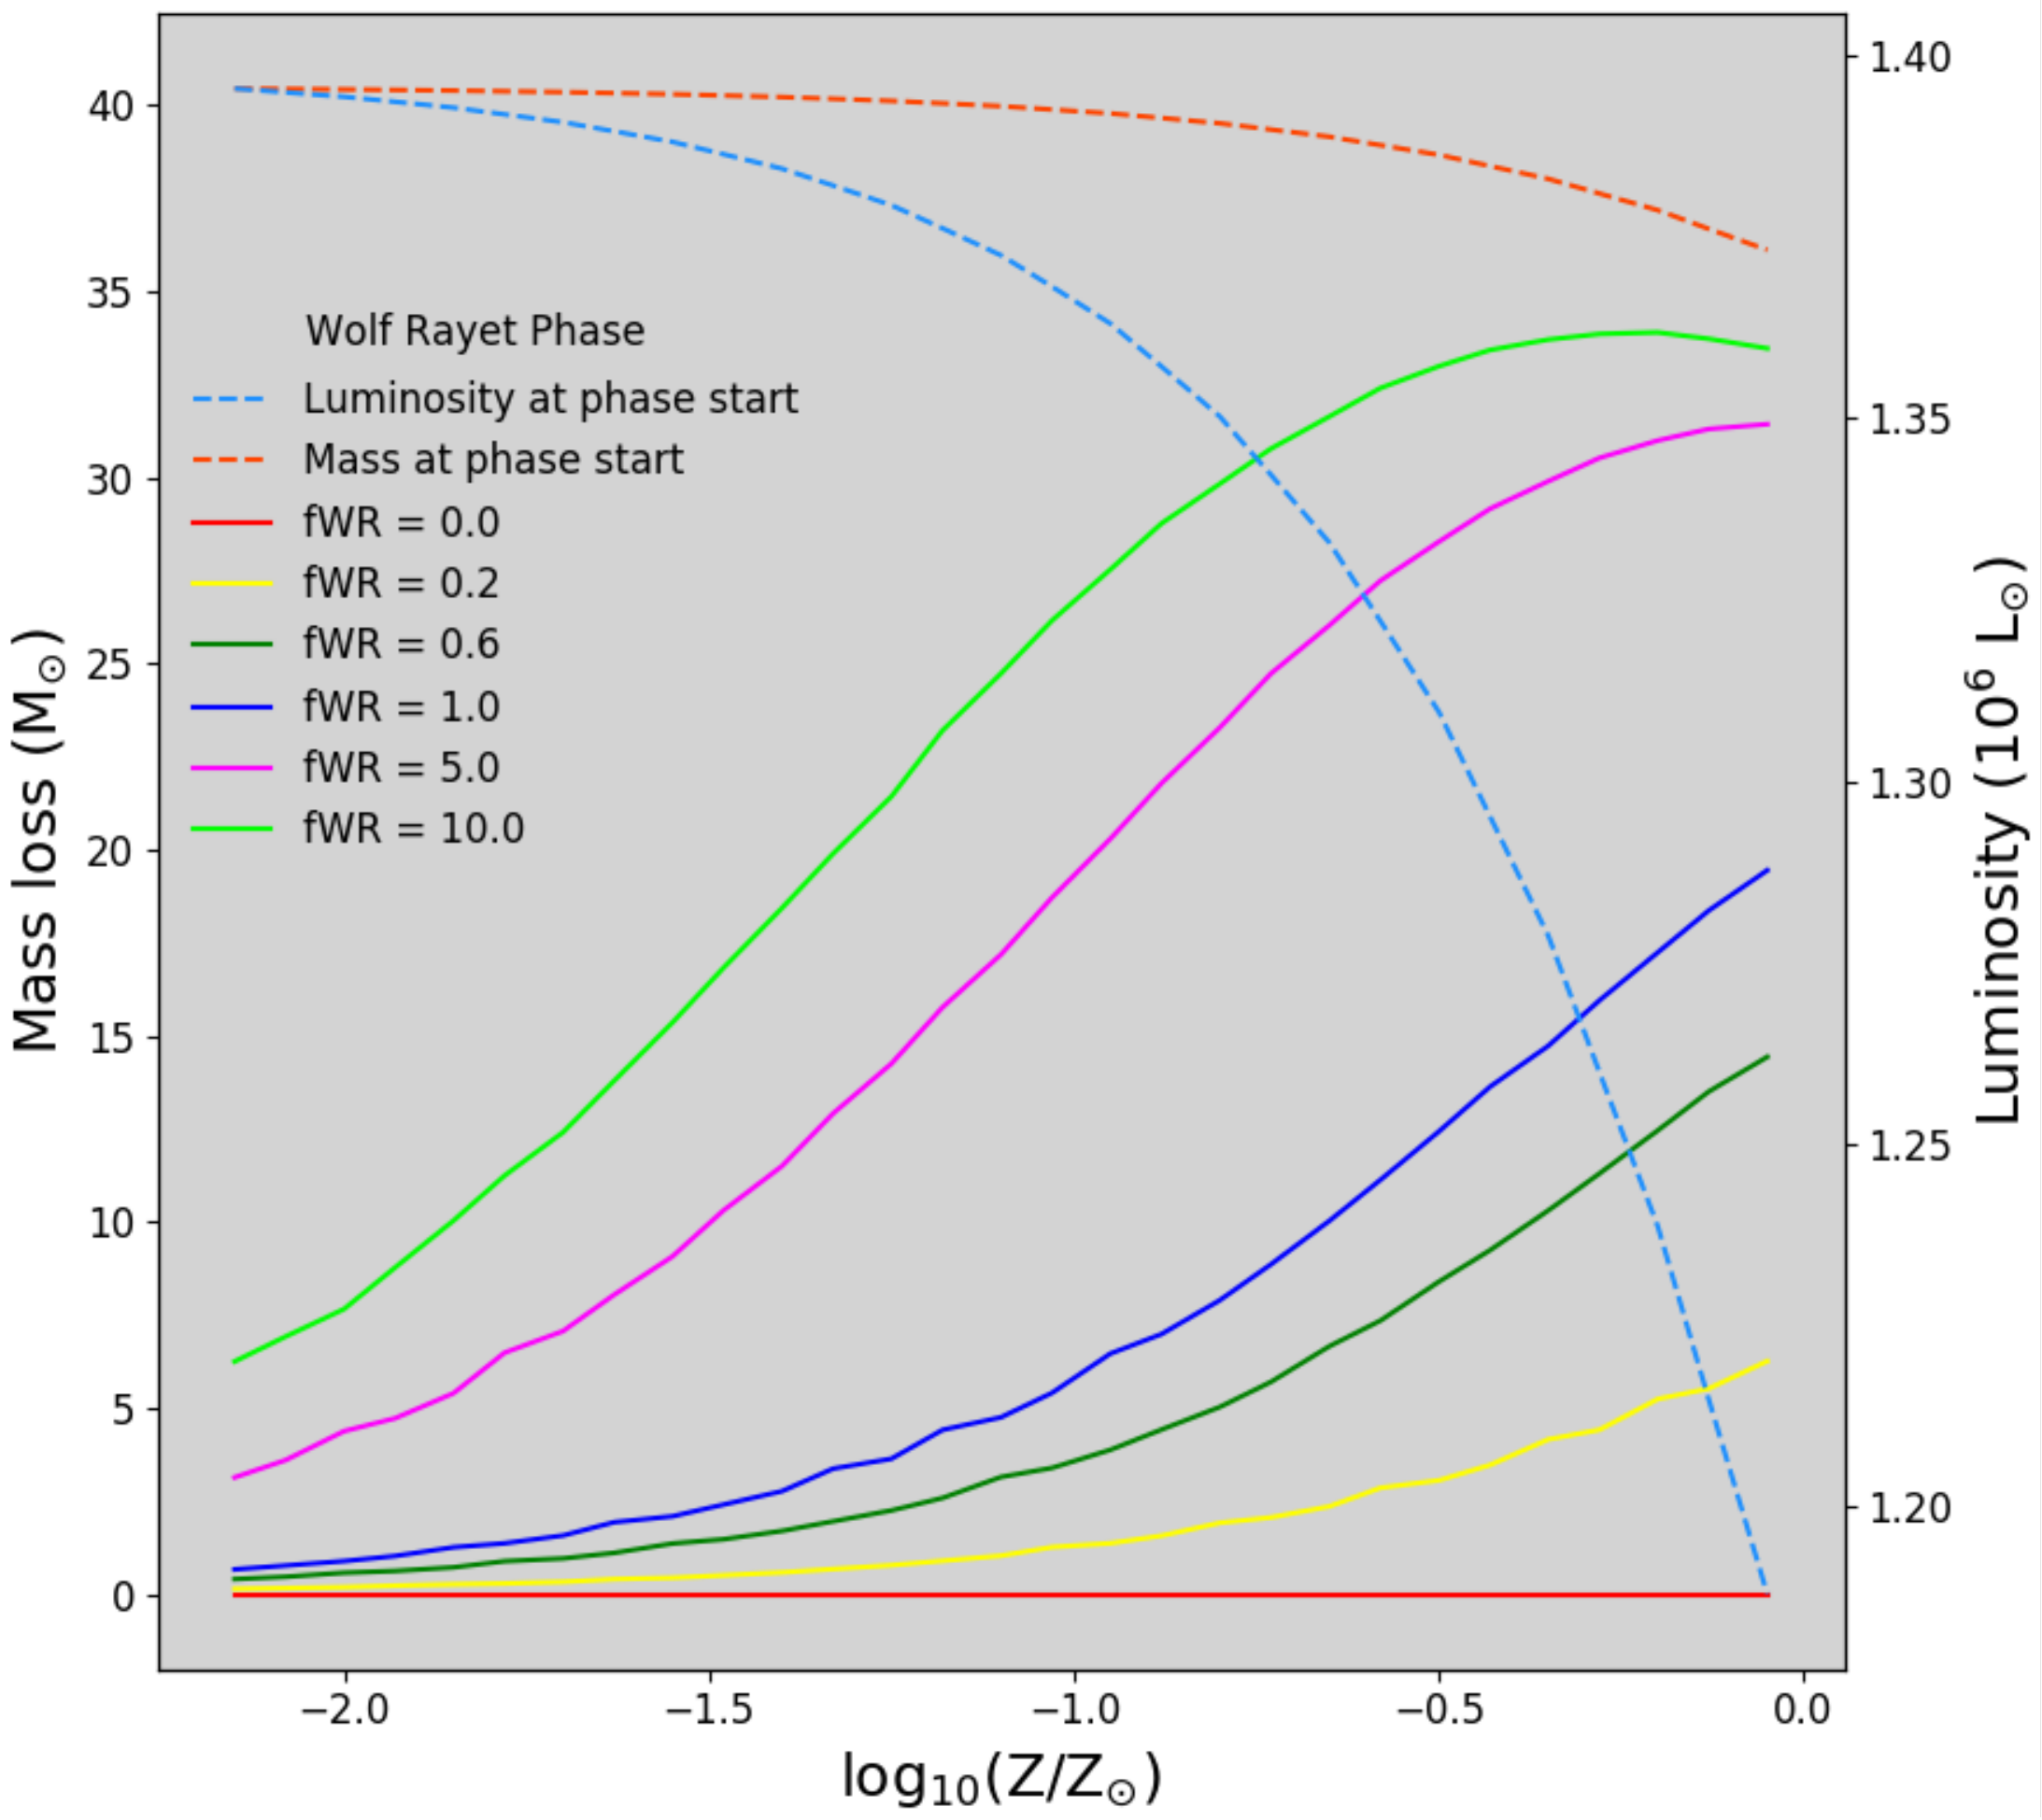}
    \captionof{figure}{Total mass lost by a \ac{WR} star with a \ac{ZAMS} mass of $40.5 \Msun$ as a function of metallicity. Line colour indicates the \ac{WR} mass loss rate multiplier (solid lines). Also shown are the mass (on the same scale as the mass loss curves) and luminosity at the start of the \ac{WR} phase as a function of metallicity (dashed lines).}
    \label{fig:WRActualMassLoss}
\end{minipage}

\jeff{Since one of the initial goals was to see the effect of varying WR winds, should we bring this discussion into the main body, or leave it in the appendix?}
\avg{[I think you should incorporate it and the discussion in the main body. It might make the main text longer, but I think you can reduce the explanation and make the overall document shorter. It is worth including and discussing.]}
\avg{[The only appendix you really need is that describing Ellen's work.]}
\end{multicols}
\twocolumn
